# Supplementary material for: Distributional Treatment Effect Transportability across Heterogeneous Sites
Source: arXiv:2511.09759 source file (2026-09-03)
Supplement: Supplementary file 1 [file final_appendix.tex]

\PassOptionsToPackage{table,xcdraw}{xcolor}
\documentclass[12pt]{article}
\input{final_preamble}

\setcounter{figure}{2}
\setcounter{table}{3}

\begin{document}
\def\spacingset#1{\renewcommand{\baselinestretch}%
{#1}\small\normalsize} \spacingset{1}

% Moderate, robust display-math spacing (survives class/package resets)
\makeatletter
\g@addto@macro\normalsize{%
  \setlength\abovedisplayskip{10pt plus 2pt minus 5pt}%
  \setlength\belowdisplayskip{10pt plus 2pt minus 5pt}%
  \setlength\abovedisplayshortskip{6pt plus 2pt minus 3pt}%
  \setlength\belowdisplayshortskip{6pt plus 2pt minus 3pt}%
  \setlength\jot{3pt}% line spacing inside align/eqnarray-like
}
\makeatother

{
  %\title{\bf Optimal Transport for Aligning Heterogeneous Data in Estimating Distributional Treatment Effects}
  \title{Supplementary Material for: \\ Distributional Treatment Effect Estimation across Heterogeneous Sites via Optimal Transport}
\author{ Borna Bateni\\
Department of Statistics \& Data Science, University of California, \\ Los Angeles, Los Angeles, CA, USA\\
Yubai Yuan\\
Department of Statistics, The Pennsylvania State University, \\ University Park, PA, USA\\
Qi Xu\\
Department of Statistics \& Data Science, Carnegie Mellon University, Pittsburgh, PA, USA\\
and \\
Annie Qu\thanks{
    Corresponding author. E-mail: \texttt{aqu2@ucsb.edu}. 
    The authors gratefully acknowledge support from the U.S. National Science Foundation (NSF) under Grants DMS-2515275 and DMS-2515698.
  }\\
Department of Statistics \& Applied Probability, University of California, Santa Barbara, Santa Barbara, CA, USA
}

  \date{}
  \maketitle
  \vspace{-10mm}

}
\spacingset{1.7}
\appendix
\section{Proofs and additional Lemmas}
We begin with a basic lemma establishing that the pull-back metric induced by a bijective mapping between the source and target spaces is indeed a proper metric.

\begin{lemma}\label{lem:1}
For any bijective mapping $\phi:\Z\to\Z'$ from the source to the target space, the pull-back metric define as: $$ d_\phi'(z_1',z_2') = d_Z(\phi^{-1}(z_1'),\phi^{-1}(z_2'))\foral z_1',z_2'\in\Z'.$$ constitutes a proper metric on $\Z'$.
\end{lemma}

\begin{proof}[Proof of Lemma \ref{lem:1}]
Symmetry and Triangle inequality of $d_\phi'$ follow directly from the corresponding properties of the original metric $d_Z$ and well-definedness of $\phi$. Positivity follows from the bijectivity of $\phi$: if $z'_1\neq z'_2\in\Z'$ then by injectivity of $\phi$, $\phi^{-1}(z'_1)\neq \phi^{-1}(z'_2)$, and by the positivity of the metric $d_Z$, we have $d'_\phi(z'_1,z'_2)=d_Z(\phi^{-1}(z'_1),\phi^{-1}(z'_2))>0$.
\end{proof}

\subsection{Proof of Lemma 3.1} \label{proof:lem3}
\begin{proof}[Proof of Lemma 3.1] 

We divide the argument into two stages: the continuous case corresponding to the population-level setting, and second, its empirical `discrete' realization.

\paragraph{(i)} In the first stage, we consider the idealized setting in which the control measures $\mu_0$ and $\mu'_0$ on $\Z$ and $\Z'$ are observed in their entirety. Accordingly, the loss terms are naturally redefined as: 
$$\mathscr L_{\FGW_\alpha}(\pi,d'_\phi)=\int_{\Z\times\Z'}\!\int_{\Z\times\Z'}\!\Bigl((1-\alpha)\,\mathcal K(z_1,z'_1)
          +\alpha\,\bigl|d_Z(z_1,z_2)-d'_\f(z'_1,z'_2)\bigr|\Bigr)
   \,d\pi_\f(z_1,z'_1)\,d\pi_\f(z_2,z'_2), $$ and $$\mathscr L_G(\pi,d'_\phi)=\int_{\Z\times\Z'}\! d'_\phi(\phi(z_1),z'_1)\; d\pi(z_1,z'_1).$$ 

For the deterministic coupling  
$${\pi}_{\f} = (\text{Id},\f)_{\#}{\mu_0}\; :B \mapsto \mu_0\big(\{z\in \Z: (z,\f(z))\in B\}\big),\,\text{for any $B\in \sigma(\Z\times\Z')$\;,}$$ and since \(\mu_0' = \f_{\#}{\mu_0}\) by
Assumption 3.1, we have for any
\(g \in L^1\bigl([\Z\times\Z']^2\bigr)\):
\[
\eqbox{
\int_{\Z\times\Z'}\!\!\int_{\Z\times\Z'} g\bigl((z_1,z'_1),(z_2,z'_2)\bigr)
\,d\pi_\f(z_1,z'_1)\,d\pi_\f(z_2,z'_2)
\;=\;
\int_\Z\!\!\int_\Z g\bigl((z_1,\f(z_1)),(z_2,\f(z_2))\bigr)
\,d\mu_0(z_1)\,d\mu_0(z_2).
}
\]

Hence, for the fused Gromov–Wasserstein loss,
\[
\eqbox{
\begin{aligned}
\mathscr L_{\FGW_\alpha}(\pi_\f,d'_\f)
&= \int_{\Z\times\Z'}\!\!\int_{\Z\times\Z'}
   \Bigl[(1-\alpha)\,\mathcal K(z_1,z'_1)
          +\alpha\,\bigl|d_Z(z_1,z_2)-d'_\f(z'_1,z'_2)\bigr|\Bigr]
   \,d\pi_\f(z_1,z'_1)\,d\pi_\f(z_2,z'_2) \\[2pt]
&= \int_\Z\!\!\int_\Z
   \Bigl[(1-\alpha)\,\mathcal K\bigl(z_1,\f(z_1)\bigr)
          +\alpha\,\bigl|d_Z(z_1,z_2)-d'_\f\bigl(\f(z_1),\f(z_2)\bigr)\bigr|\Bigr]
   \,d\mu_0(z_1)\,d\mu_0(z_2).
\end{aligned}}
\]

By definition of the pull-back metric,
\(d'_\f\bigl(\f(z_1),\f(z_2)\bigr)=d_Z(z_1,z_2)\), so the
Gromov–Wasserstein term vanishes.
Moreover, Assumption 3.2 ensures that the alignment term satisfies
\(\mathcal K\!\bigl(z_1,\f(z_1)\bigr)=0\),
making the pair  
\((\pi_\f,d'_\f)\) achieve zero FGW loss. It is also immediate that the pair \((\pi_\f,d'_\f)\) yields zero graph-consistency penalty as well, and thus lies in the zero-level set of the regularized objective:
\[
\mathscr L_{\FGW_\alpha}\bigl(\pi_\f,d'_\f\bigr) + \lambda\cdot \mathscr L_G(\pi_\f, d'_\f)=0.
\]

Conversely, assume that there exists another pair of coupling and metric, $( \widetilde{\pi}, \dtwo)$ satisfying $\mathscr L_{\FGW_\alpha}\bigl(\widetilde{\pi}, \dtwo\bigr) + \lambda\cdot \mathscr L_G(\widetilde{\pi}, \dtwo)=0$. By the ``if and only if" quality of Proposition 3 of \citet{vayer2020fused}, there should exist a bijection $\ftwo:\Z\to\Z'$ with $\ftwo_{\#}{\mu_0}=\mu_0'$ such that the metric $\dtwo$ is a pullback: $\dtwo=d'_{\ftwo}:(z'_1,z'_2)\mapsto d_Z(\ftwo^{-1}(z'_1), \ftwo^{-1}(z'_2))$. Thus, similar to the above, for the deterministic coupling $\pi_\ftwo = (\text{Id}, \ftwo)_\#\mu_0\in \Pi(\mu_0,\mu_0')$ we should have $\mathscr L_{\FGW_\alpha}\bigl({\pi_\ftwo}, d'_\ftwo\bigr)=0$ as well. Evaluating the FGW loss under \(( \pi_{\ftwo},d'_\ftwo)\) and using the marginal
relations \(\ftwo_{\#}\mu_0=\mu_0'\) and  \(\f_{\#}\mu_0=\mu_0'\),  we get
\[
\eqbox{
\begin{aligned}
0
&= \mathscr L_{\FGW_\alpha}(\pi_{\ftwo},d'_{\ftwo}) \\[2pt]
&= \int_{\Z\times\Z'}\!\!\int_{\Z\times\Z'}
   \Bigl[(1-\alpha)\,\mathcal K(z_1,z'_1)
          +\alpha\,\bigl|d_Z(z_1,z_2)-d'_{\ftwo}(z'_1,z'_2)\bigr|\Bigr]
   \,d\pi_{\ftwo}(z_1,z'_1)\,d\pi_{\ftwo}(z_2,z'_2) \\[4pt]
&\ge \int_{\Z\times\Z'}\!\!\int_{\Z\times\Z'}
      \alpha\,\bigl|d_Z(z_1,z_2)-d'_{\ftwo}(z'_1,z'_2)\bigr|
   \,d\pi_{\ftwo}(z_1,z'_1)\,d\pi_{\ftwo}(z_2,z'_2) \\[4pt] \text{(since $\ftwo_{\#}\mu_0=\mu_0'$)}\qquad
&=   \int_{\Z}\!\int_{\Z\times\Z'}
      \alpha\,\bigl|d_Z(z_1,z_2)-d'_{\ftwo}(\ftwo(z_1),z'_2)\bigr|
   \,d\mu_{0}(z_1)\,d\pi_{\ftwo}(z_2,z'_2) \\[4pt] \text{(since $\f_{\#}\mu_0=\mu_0'$)}\qquad
&= \int_{\Z}\!\int_{\Z}
      \alpha\,\bigl|d_Z(z_1,z_2)-d'_{\ftwo}\bigl(\ftwo(z_1),\f(z_2)\bigr)\bigr|
   \,d\mu_0(z_1)\,d\mu_0(z_2) \\[4pt]
&= \int_{\Z}\!\int_{\Z}
      \alpha\,\bigl|d_Z(z_1,z_2)-d_Z\bigl(z_1,\ftwo^{-1}\circ\f(z_2)\bigr)\bigr|
   \,d\mu_0(z_1)\,d\mu_0(z_2).
\end{aligned}}
\]
Since $\Z$ is Polish, $\mu_0$ is a Radon measure and Fubini's theorem applies. Hence, for $\mu_0$ - almost every $z_1\in \Z$: 
\begin{equation}\label{eq:penul}d_Z(z_1,z_2)=d_Z(z_1,\ftwo^{-1}\circ \f(z_2)),\qquad \text{for $\mu_0$-a.e. }z_2\in \Z. \end{equation}

Define, for each $z_2\in \Z$, the function  $f_{z_2}:z_1\mapsto d_Z(z_1,z_2) - d_Z(z_1,\ftwo^{-1}\circ\f(z_2))$.
By Triangle inequality, $z_1\mapsto d_Z(z_1,z_2)$ is 1-Lipschitz and continuous for every $z_2\in \Z$. Thus, each $f_{z_2}$ is continuous in its argument $z_1$. 

By \eqref{eq:penul}, $f_{z_2}=0$ for $\mu_0$ - almost every $z_2\in \Z$. Let: $$S:=\{z\in\Z: \mu_0(f_z^{-1}(0))=1\}\;,$$ so that $\mu_0(S)=1$. Define the subset $\widetilde S= \{ z\in S: \ftwo^{-1}\circ \f({{z}})\neq {{z}}\}$ and choose any  $\tilde z\in \tilde S$ with  $\delta_{\tilde{z}}:=d_Z({\tilde{z}},\ftwo^{-1}\circ \f({\tilde{z}}))>0$. For every $z\in f_{\tilde z}^{-1}(0)$ we have $d_Z(z,\tilde z)=d_Z(z,\ftwo^{-1}\circ \f(\tilde z))$, and the triangle inequality gives: $$ \begin{aligned}
d_Z(z,\tilde z)=\dfrac{d_Z(z,\tilde z) + d_Z({z},\ftwo^{-1}\circ \f({\tilde{z}}))}{2}&\geq \dfrac{d(\tilde{z},\ftwo^{-1}\circ \f({\tilde{z}}))}{2}
\\&= \delta_{\tilde z}/2=:r_{\tilde z}>0\;,\qquad \text{for all }z\in f_{\tilde z}^{-1}(0).
\end{aligned}$$ Accordingly, $f_{\tilde z}^{-1}(0)\cap B_{r_{\tilde z}}(\tilde z)=\emptyset$ and in order for $\tilde z\in \tilde S\subseteq S$ to have $\mu_0(f_{\tilde z}^{-1}(0))=1$, we need: $$\mu_0(B_{r_{\tilde z}}(\tilde z))=0\;.$$ The set of all such balls, $\bigcup_{\tilde z\in \widetilde S} B_{r_{\tilde z}}(\tilde z)$, covers $\widetilde S$. Also, $\Z$ is a metric space, hence second countable and Lindel\"{o}f. Hence, the open cover $\bigcup_{\tilde z\in \widetilde S} B_{r_{\tilde z}}(\tilde z)$ admits a countable subcover $\bigcup_{m\in\mathbb N}B_{r_{\tilde z_m}}(\tilde z_m)$, and by countable subadditivity of measure:$$ \mu_0(\widetilde S)\leq\mu_0\bigl(\bigcup_{m\in \mathbb N} B_{r_{\tilde z_m}}(\tilde z_m)\bigr)\leq  \sum_{m\in \mathbb N}\mu_0(B_{r_{\tilde z_m}}(\tilde z_m))=0\;,$$ and accordingly: $$\{z\in \Z: \ftwo^{-1}\circ \f(z)=z\}\supseteq S\setminus \tilde S\implies \mu_0(\{z\in \Z: \ftwo^{-1}\circ \f(z)=z\})\geq \mu_0(S)-\mu_0(\widetilde S)=1\;,$$

Hence it follows that: \begin{equation}\ftwo= \f\qquad \mu_0 \text{ - almost everywhere.}\label{eq: T=T' a.e.}\end{equation}

Lastly, it remains to show that the coupling $\widetilde \pi$ is uniquely determined and coincides with the deterministic coupling $\pi_{\f} := (\text{Id},\f)_\# \mu_0$ almost everywhere.

Define the \emph{graph} of $\ftwo$, 
\(
G_{\ftwo}:=\bigl\{(z,\ftwo(z)):z\in\Z\bigr\}\subseteq\Z\times\Z',
\)
and its complement
$K_{\ftwo}:=(\Z\times\Z')\setminus G_{\ftwo}$.
Because the graph–consistency loss vanishes,
\[
\mathscr L_G(\widetilde\pi,d'_{\ftwo})
=\int_{\Z\times\Z'}d'_{\ftwo}\!\bigl(\ftwo(z_1),z'_1\bigr)
  \,d\widetilde\pi(z_1,z'_1)
=0.
\]

For $k\in\mathbb N$ set
\[
K_{\ftwo}^{(k)}
=\Bigl\{(z,z')\in K_{\ftwo}:
      d'_{\ftwo}\!\bigl(\ftwo(z),z'\bigr)>\tfrac1k \Bigr\},
\qquad
K_{\ftwo}= \bigcup_{k=1}^{\infty}K_{\ftwo}^{(k)}.
\]
By monotone convergence,
\[\begin{aligned}
0
&= \int_{\Z\times\Z'}d'_{\ftwo}\!\bigl(\ftwo(z_1),z_2\bigr)
  \,d\widetilde\pi(z_1,z'_1)\\
  &\geq\int_{K_{\ftwo}^{(k)}}d'_{\ftwo}\bigl(\ftwo(z_1),z_1'\bigr)
    \,d\widetilde\pi
\;\ge\;
\frac1k\,\cdot\,\widetilde\pi\bigl(K_{\ftwo}^{(k)}\bigr),
\quad k\in\mathbb N, \end{aligned}
\]
so each $K_{\ftwo}^{(k)}$ has $\widetilde\pi$–measure zero.  Taking the
countable union yields
\[
\widetilde\pi\!\bigl(K_{\ftwo}\bigr)=0\;,
\]
meaning $\widetilde\pi$ is supported on $G_{\ftwo}$. 
Hence: \begin{equation}\label{eq: pi=pi_T}\widetilde\pi=({G_{\ftwo}})_{\#}\mu_0=\pi_{\ftwo}=\pi_\f\;.\end{equation}

\paragraph{(ii)} 

For the discrete case, fix i.i.d.\ sequences $Z_0:=\{z_{0i}\}_{i\ge1}\sim\mu_0$ and $Z_0':=\{z'_{0k}\}_{k\ge1}\sim\mu_0'$, and let
$\widehat\mu_0^{(n_0)}\!:=\frac1{n_0}\sum_{i=1}^{n_0}\delta_{z_{0i}}$ and
$\widehat\mu_0'^{(n_0')}\!:=\frac1{n_0'}\sum_{k=1}^{n_0'}\delta_{z'_{0k}}$ denote the empirical measures formed from their first $n_0$ and $n_0'$ observations, respectively.
Since $\Z$ is Polish, by Varadarajan’s theorem \citep[Theorem~11.4.1]{dudley2002real}, there exists an event
\[
\Omega_{\mathrm{emp}}\in\mathcal F,\qquad \mathbb P(\Omega_{\mathrm{emp}})=1,
\]
such that on $\Omega_{\mathrm{emp}}$ we have
$\widehat\mu_0^{(n_0)}\stackrel{w}{\longrightarrow}\mu_0$ and
$\widehat\mu_0'^{(n_0')}\stackrel{w}{\longrightarrow}\mu_0'$ as $n_0,n_0'\to\infty$.
By the \cite{kuratowski1965selectors} measurable selection theorem, we can fix a measurable selector
\[
(\widehat\pi^*_{n_0,n_0'},\phi^*_{n_0,n_0'})\in\arg\min_{\hpi\in\Pi(\widehat\mu_0^{(n_0)},\widehat\mu_0'^{(n_0')}),\ \phi\in\Phi}
\Big\{\mathscr L_{\FGW_\alpha}(\hpi,d'_\phi)+\lambda\,\mathscr L_G(\hpi,d'_\phi)\Big\}.
\]
Set $\Omega^\star\!:=\Omega_{\mathrm{emp}}$. In what follows we fix an arbitrary $\omega\in\Omega^\star$ and suppress the dependence on $\omega$; all limits are then deterministic along this sample path.

By Theorem~2 of \citet{vayer2020fused}, for the empirical measures
\(\mh_0^{(n_0)},\mh_0'^{(n_0')}\), and any valid target metric $d'_Z$ we have
\[
\FGW_{1,1,\alpha}(\mh_0^{(n_0)},\mu_0|d'_Z)\xrightarrow[n_0\to\infty]{}0,
\qquad
\FGW_{1,1,\alpha}(\mh_0'^{(n_0')},\mu_0'|d'_Z)\xrightarrow[n_0'\to\infty]{}0.
\]
Hence, for the pull-back metric \(d'_{\f}\), the triangle inequality yields
\[\eqbox{
\begin{aligned}
\inf_{\hpi\in\Pi(\mh_0^{(n_0)},\mh_0'^{(n_0')})}
\mathscr L_{\FGW_\alpha}(\hpi,d'_{\f}) &=
{\FGW_{1,1,\alpha}(\mh_0^{(n_0)},\mh_0'^{(n_0')}|d'_\f)}\\
&\le 
\FGW_{1,1,\alpha}(\mu_0,\mh_0^{(n_0)}|d'_\f)
+\FGW_{1,1,\alpha}(\mu_0',\mh_0'^{(n_0')}|d'_\f)
+{\FGW_{1,1,\alpha}(\mu_0,\mu_0'|d'_\f)} \\[2pt]
\xrightarrow[]{n_0,n_0'\to\infty} 
&\;\;\;\;\;{\FGW_{1,1,\alpha}(\mu_0,\mu_0'|d'_\f)}\\
&=\mathscr L_{\FGW_\alpha}(\pi_\f,d_\f') = 0 \qquad \text{(by (i)).}
\end{aligned}}
\]

Now, under any other target metric $\dtwo\neq d'_\f$, the triangle inequality yields
\[\eqbox{
\begin{aligned}
\inf_{\hpi\in\Pi(\mh_0^{(n_0)},\mh_0'^{(n_0')})}
\mathscr L_{\FGW_\alpha}(\hpi,\dtwo) &=
{\FGW_{1,1,\alpha}(\mh_0^{(n_0)},\mh_0'^{(n_0')}|\dtwo)}\\
&\ge {\FGW_{1,1,\alpha}(\mu_0,\mu_0'|\dtwo)} 
-\FGW_{1,1,\alpha}(\mu_0,\mh_0^{(n_0)}|\dtwo)
-\FGW_{1,1,\alpha}(\mu_0',\mh_0'^{(n_0')}|\dtwo)
\\[2pt]
\xrightarrow[]{n_0,n_0'\to\infty} 
&\;\;\;\;\;{\FGW_{1,1,\alpha}(\mu_0,\mu_0'|\dtwo)}\\
&=\inf_{\pi\in\Pi(\mu_0,\mu'_0)}\mathscr L_{\FGW_\alpha}(\pi,\dtwo) \;,
\end{aligned}}
\] where $\inf_{\pi\in\Pi(\mu_0,\mu'_0)}\mathscr L_{\FGW_\alpha}(\pi,\dtwo)$ is proven in part (i) to be strictly positive, unless $\dtwo$ is itself a pullback metric, $\dtwo=d'_\ftwo$, and $\ftwo = \f$, $\mu_0$-almost everywhere. Therefore, $d'_\f$ is the unique metric (up to $\mu_0$- null sets) that asymptotically achieves zero empirical FGW loss.

For the remainder of the proof, we fix the pull-back metric $d'_\f$, and assume $\mathcal K\in C_b(\Z\times \Z')$ and $ d_Z\in C_b(\Z\times \Z)$. This entails no substantive loss of generality: continuity of $d_Z$ is inherent; for boundedness, we may replace any metric $d$ (or kernel) by a topologically equivalent bounded metric $\bar d(z_1,z_2):= \psi(d(z_1,z_2))$, with a strictly increasing, continuous $\psi$ such as $\psi(t) = \tanh(t)$. Moreover, under Assumption 3.1, $\f$ is bi-measurable, so $d'_{\f}(z'_1,z'_2)=d_Z(\f^{-1}(z'_1),\f^{-1}(z'_2))$ is Borel measurable, and by Lusin’s theorem \cite[Theorem~7.1.13]{bogachev2007measureI}, for every $\varepsilon>0$
there exists a compact $K'\subset \Z'$ with $\mu_0'(K')>1-\varepsilon$ such that
$\f^{-1}$ is continuous on $K'$, hence $d'_{\f}$ is continuous on $K'\times K'$. Consequently, the FGW integrand  $$F_\alpha(z_1,z'_1,z_2,z'_2):=\Bigl[(1-\alpha)\,\mathcal K(z_1,z'_1)
          +\alpha\,\bigl|d_Z(z_1,z_2)-d'_{\f}(z'_1,z'_2)\bigr|\Bigr]\;,$$ is bounded and measurable on $(\Z\times\Z')^2$, and is continuous on
$(K\times K')^2$ for any compact $K\subset\Z$ and the $K'$ given above.

Assume there exists a sequence \(\{\widehat\pi_{n_0,n_0'}\}_{n_0,n_0'\in\mathbb N}\), with each
\(\widehat\pi_{n_0,n_0'}\in \Pi\big(\widehat\mu_0^{(n_0)},\widehat\mu_0'^{(n_0')}\big)\), that converges weakly to the coupling \(\pi_\infty\in \Pi(\mu_0,\mu'_0)\),
\(\widehat\pi_{n_0,n_0'}\xrightarrow[]{w} \pi_{\infty}\) as \(n_0,n_0'\to\infty\), meaning
\[
\int_{\mathcal Z\times\mathcal Z'} \Phi\, d\widehat\pi_{n_0,n_0'}
\;\longrightarrow\;
\int_{\mathcal Z\times\mathcal Z'} \Phi\, d\pi_{\infty}
\qquad\text{for all }\; \Phi\in C_b(\mathcal Z\times\mathcal Z')\;.
\]

Since $\Z\times \Z'$ is Polish, and  $\hpi_{n_0,n'_0}\xrightarrow[]{w}\pi_\infty$, by Prokhorov's Theorem \citep[Theorem~8.6.2]{bogachev2007measureII} the sequence is \emph{uniformly tight}, meaning for any $\varepsilon>0$, there exists a compact $K\in \Z\times\Z'$, such that 
\begin{equation}\label{eq:K^c}\sup_{n_0,n'_0\in\mathbb N}\hpi_{n_0,n'_0}(K^\complement) \lor \pi_\infty(K^\complement)<\varepsilon\;.\end{equation}
Consider the compact product $K\times K\subseteq (\Z\times\Z')^2$. By the general Stone-Weierstrass theorem \citep[Theorem~7.32]{rudin1976principles}, the algebra generated by functions of the form $(x,y)\mapsto f(x)\cdot g(y)$ with $f,g\in C_b(\Z\times\Z')$ is uniformly dense in $C(K\times K)$. Therefore, for any arbitrary $\Phi \in C_b((\Z\times\Z')^2)$, and any $\varepsilon>0$, there exists a $$\widetilde \Phi:(x,y)\mapsto \sum_{j=1}^J f_j(x)\cdot g_j(y)\;,\qquad f_j,g_j\in C_b(\Z\times\Z')\;,$$ such that \begin{equation}\label{eq:supPhi}\sup_{(x,y)\in (\Z\times\Z')^2} |\Phi(x,y)-\widetilde\Phi(x,y)|< \varepsilon\;.\end{equation}

Combining \eqref{eq:K^c} and \eqref{eq:supPhi}, for any $\Phi\in C_b((\Z\times\Z')^2)$ and $\varepsilon>0$ we obtain

\[\eqbox{
\begin{aligned}
\bigg| \iint \Phi\, d(\widehat\pi_{n_0,n_0'}\!\otimes \widehat\pi_{n_0,n_0'}) 
       - \iint \Phi\, d(\pi_{\infty}\!\otimes \pi_{\infty}) \bigg|
&\le \bigg| \iint_{K\times K} \Phi\, d(\widehat\pi_{n_0,n_0'}\!\otimes \widehat\pi_{n_0,n_0'})
       - \iint_{K\times K} \Phi\, d(\pi_{\infty}\!\otimes \pi_{\infty}) \bigg| \\
&\quad + \underbrace{\bigg|\iint_{(K\times K)^\complement}\!\!\!\Phi\, d(\widehat\pi_{n_0,n_0'}\!\otimes \widehat\pi_{n_0,n_0'})\bigg|}_{\le \|\Phi\|_\infty (\,\widehat\pi_{n_0,n_0'}\!\otimes \widehat\pi_{n_0,n_0'})( (K\times K)^\complement)}
\\[-2pt]
&\quad + \underbrace{\bigg|\iint_{(K\times K)^\complement}\!\!\!\Phi\, d(\pi_{\infty}\!\otimes \pi_{\infty})\bigg|}_{\le \|\Phi\|_\infty (\,\pi_{\infty}\!\otimes \pi_{\infty})( (K\times K)^\complement)}.
\end{aligned}}
\]
Since $(\eta\otimes\eta)((K\times K)^\complement)=1-\eta(K)^2\le 2\,\eta(K^\complement)$ for any probability measure $\eta$,
\eqref{eq:K^c} gives the tail bound
\[ \sup_{n_0,n'_0\in\mathbb N}
(\widehat\pi_{n_0,n_0'}\!\otimes \widehat\pi_{n_0,n_0'})\big((K\times K)^\complement\big)
\;\vee\;
(\pi_{\infty}\!\otimes \pi_{\infty})\big((K\times K)^\complement\big)
\;\le\;2\varepsilon,
\]
and therefore
\[\eqbox{
\bigg| \iint \Phi\, d(\widehat\pi_{n_0,n_0'}\!\otimes \widehat\pi_{n_0,n_0'}) 
       - \iint \Phi\, d(\pi_{\infty}\!\otimes \pi_{\infty}) \bigg|
\;\le\; \bigg| \iint_{K\times K} \!\!\!\!\!\!\Phi\, \big[d(\widehat\pi_{n_0,n_0'}\!\otimes \widehat\pi_{n_0,n_0'})
       - d(\pi_{\infty}\!\otimes \pi_{\infty})\big] \bigg| \;+\; 4\varepsilon\|\Phi\|_\infty\;.}
\]
Next, approximate $\Phi$ on $K\times K$ by $\widetilde\Phi=\sum_{j=1}^J f_j\cdot g_j$ as in \eqref{eq:supPhi}.
Then
\[\eqbox{
\begin{aligned}
\bigg| \iint_{K\times K} \!\!\!\!\!\!\Phi\, \big[d(\widehat\pi_{n_0,n_0'}\!\otimes \widehat\pi_{n_0,n_0'})
       - d(\pi_{\infty}\!\otimes \pi_{\infty})\big] \bigg|
&\le \iint_{K\times K} |\Phi-\widetilde\Phi|\, d(\widehat\pi_{n_0,n_0'}\!\otimes \widehat\pi_{n_0,n_0'}) \\
&\quad + \iint_{K\times K} |\Phi-\widetilde\Phi|\, d(\pi_{\infty}\!\otimes \pi_{\infty}) \\
&\quad + \bigg| \iint_{K\times K} \!\!\!\!\!\!\widetilde\Phi\, \big[d(\widehat\pi_{n_0,n_0'}\!\otimes \widehat\pi_{n_0,n_0'})
       - d(\pi_{\infty}\!\otimes \pi_{\infty})\big] \bigg| \\
&\le 2\varepsilon \;+\; \bigg| \iint_{K\times K} \!\!\!\!\!\!\widetilde\Phi\, \big[d(\widehat\pi_{n_0,n_0'}\!\otimes \widehat\pi_{n_0,n_0'})
       - d(\pi_{\infty}\!\otimes \pi_{\infty})\big] \bigg|\;.
\end{aligned}}
\]

By construction of $\widetilde\Phi$, for any probability measure $\eta$ we have 
\[
\iint \widetilde\Phi\, d(\eta\otimes\eta)=\sum_{j=1}^J \Big(\int f_j\,d\eta\Big)\Big(\int g_j\,d\eta\Big).
\]
The weak convergence $\widehat\pi_{n_0,n_0'}\xrightarrow[]{w} \pi_{\infty}$ implies
\(\int f_j\,d\widehat\pi_{n_0,n_0'}\to \int f_j\,d\pi_{\infty}\) and
\(\int g_j\,d\widehat\pi_{n_0,n_0'}\to \int g_j\,d\pi_{\infty}\) for each \(j\); hence
\[
\iint \widetilde\Phi\, d(\widehat\pi_{n_0,n_0'}\!\otimes \widehat\pi_{n_0,n_0'})
\;\longrightarrow\;
\iint \widetilde\Phi\, d(\pi_{\infty}\!\otimes \pi_{\infty}).
\]
Putting the pieces together, for any $\Phi\in C_b((\Z\times\Z')^2)>0$ we obtain
\[
\limsup_{n_0,n_0'\to\infty}
\bigg| \iint \Phi\, d(\widehat\pi_{n_0,n_0'}\!\otimes \widehat\pi_{n_0,n_0'})
       - \iint \Phi\, d(\pi_{\infty}\!\otimes \pi_{\infty}) \bigg|
\;\le\; 2\varepsilon \;+\; 4\varepsilon \|\Phi\|_\infty \xrightarrow[]{\varepsilon\to 0}0.
\]
Now we apply this to the FGW integrand, $F_\alpha$. Fix $\varepsilon>0$ and choose compact $K'\subseteq \Z'$ with $\mu_0'(K')>1-\varepsilon$ such that $F_\alpha\in C_b((K\times K')^2)$ for any compact $K\subseteq \Z$. Also, choose the compact set $K= K_1\times  K_2\subseteq \Z\times \Z'$ as in \eqref{eq:K^c}, with compact components $ K_1\subseteq \Z$, $ K_2\subseteq \Z'$. 

Define the compact set $\widetilde K := K_1\times (K'\cap K_2)\subseteq \Z\times \Z'$. By Tietze's extension theorem \citep[Theorem~35.1]{munkres2000topology}, extend $F_\alpha\cdot \1_{\widetilde K^2}$ to a bounded continuous function
$\Phi_\varepsilon\in C_b((\Z\times\Z')^2)$ that coincides with $F_\alpha$ on
$(\widetilde K)^2$. Applying the previous display to $\Phi_\varepsilon$
and controlling the complement by the tightness bound \eqref{eq:K^c} together with
$\pi_{\infty}(\Z\times (K')^\complement)\le \varepsilon$, we obtain \begin{equation}
\label{eq:LFGW_conv}
\eqbox{
\mathscr L_{\FGW_\alpha}\big(\widehat\pi_{n_0,n_0'},d'_{\f}\big)
=\iint F_\alpha\, d(\widehat\pi_{n_0,n_0'}\!\otimes \widehat\pi_{n_0,n_0'})
\;\xrightarrow[]{n_0,n'_0\to \infty}\;
\iint F_\alpha\, d(\pi_{\infty}\!\otimes \pi_{\infty})
=\mathscr L_{\FGW_\alpha}\big(\pi_{\infty},d'_{\f}\big).}
\end{equation}

Next, consider the graph-consistency loss $$\mathscr L_G(\pi, d'_\f)=\int_{\Z\times \Z'} d_Z(z,\f^{-1}(z'))\;d\pi(z,z')\;.$$ we know the graph-consistency cost $g:(z,z')\mapsto d_Z(z,\f^{-1}(z'))$ is bounded and measurable by $d_Z\in C_b(\Z\times\Z)$ and bi-measurability of $\f$. Let $D_g$ denote the discontinuity set of $g$. Since $z\mapsto d_Z(z,.)$ is continuous, we have $D_g=\Z\times D_{\f^{-1}}$. Since both $\Z$ and $\Z'$ are polish and $\mu_0,\mu_0'$ are finite (probability) measures, by Lusin's theorem \citep[Theorem~7.1.13]{bogachev2007measureI}, for any arbitrary $\varepsilon>0$ there exists a compact $K\subseteq \Z'$ with $\mu_0'(K)>1-\varepsilon$ such that $\f^{-1}$ is continuous on $K$. Thus for any coupling $\pi_\infty \in \Pi(\mu_0,\mu'_0)$ we have $$\pi_\infty(D_g) = \pi(\Z\times D_{\f^{-1}})= \mu_0'(D_{\f^{-1}})\leq \mu_0'(\Z'\setminus K)<\varepsilon\xrightarrow{\varepsilon\to0}0\;,$$ meaning $g$ is $\pi_\infty$-almost everywhere continuous. Accordingly, by the Portmanteau theorem \citep[Theorem~2.1(v)]{billingsley1999convergence} we obtain
\begin{equation}
    \label{eq:LG_conv}\mathscr L_G(\hpi_{n_0,n'_0},d'_\f)=\int_{\Z\times\Z'} g\;d\hpi_{n_0,n'_0}\xrightarrow[]{n_0,n'_0\to\infty} \int_{\Z\times\Z'} g\;d\pi_{\infty}=\mathscr L_G(\pi_{\infty},d'_\f)\;.
\end{equation}

\eqref{eq:LFGW_conv} and \eqref{eq:LG_conv} yield that the total loss $Q:\pi\mapsto\mathscr L_{\FGW_\alpha}(\pi,d'_{\f})+\lambda\,\mathscr L_G(\pi,d'_{\f})$ is continuous with respect to the weak convergence of couplings: if \(\widehat\pi_{n_0,n_0'}\xrightarrow{w}\pi\), then \(Q(\widehat\pi_{n_0,n_0'})\to  Q(\pi)\).
By part~(i), \( Q(\pi)\ge 0\) for all \(\pi\in \Pi(\mu_0,\mu'_0)\), with a {unique} minimizer
\(\pi_{\f}\) and \(Q(\pi_{\f})=0\), while \(Q(\tilde\pi)>0\) for every \(\tilde\pi\neq\pi_{\f}\). Consequently:
 if \(\widehat\pi_{n_0,n_0'}\xrightarrow{w} \pi_{\f}\), then
\(Q(\widehat\pi_{n_0,n_0'})\to Q(\pi_{\f})=0\);
and if \(\widehat\pi_{n_0,n_0'}\xrightarrow{w} \tilde\pi\neq \pi_{\f}\) or \(\{\widehat\pi_{n_0,n_0'}\}\) has more than one weak limit, then at least one
subsequence converges to some \(\tilde\pi\neq\pi_{\f}\), hence $
\limsup_{n_0,n_0'\to\infty}\,Q(\widehat\pi_{n_0,n_0'})\;\ge\;Q(\tilde\pi)\;>\;0.
$

Lastly, it remains to \emph{exhibit} a sequence of empirical couplings that converges weakly to $\pi_\f$. For the sequence of empirical source control measures $\{\mh_0^{(n_0)}\}_{n_0\in\mathbb N}$, define the deterministic couplings $$\gamma_\f^{(n_0)}:=(\text{Id}, \f)_\#\mh_0^{(n_0)} \in \Pi(\mh_0^{(n_0)}, \widehat\nu_0^{(n_0)});\qquad \widehat\nu_0^{(n_0)} = \f_\#\mh_0^{(n_0)}\stackrel w\longrightarrow \mu_0'\;.$$ 
Since both sequences $\{\widehat\nu_0^{(n_0)}\}_{n_0\in\mathbb N}$ and $\{\mh_0'^{(n'_0)}\}_{n'_0\in\mathbb N}$ converge weakly to $\mu_0'$, their Prokhorov metric, $\rho(\widehat\nu_0^{(n_0)},\mh_0'^{(n_0')})$, tends to zero (Because the Prokhorov metric metrizes weak convergence on Polish spaces). Accordingly, by Strassen-Dudley's Theorem in the tight case \citep[Theorem~11.6.2]{dudley2002real}, there exists a sequence of couplings $\widehat{\;\varsigma\;}_{n_0,n'_0}\in \Pi(\widehat\nu_0^{(n_0)},\mh_0'^{(n'_0)})$ such that $$
\widehat{\;\varsigma\;}_{n_0,n'_0}\left(\!\left\{(z'_1,z_2')\in \Z'\times\Z' : d_{\f}'(z'_1,z_2')>\rho(\widehat\nu_0^{(n_0)},\mh_0'^{(n_0')})\right\}\right)\xrightarrow[]{n_0,n'_0\to\infty}0\;.$$ Now, define a sequence of couplings on $\Z\times\Z'$ by pushing $\widehat{\;\varsigma\;}_{n_0,n'_0}$ forward through $\f^{-1}$ on the first coordinate
\[
\hpi_{n_0,n'_0} \;\defeq\; (\f^{-1}\times \mathrm{Id})_{\#}\widehat{\;\varsigma\;}_{n_0,n'_0} \;\in\; \Pi\!\big(\mh_0^{(n_0)},\mh_0'^{(n_0')}\big).
\] By construction, the sequence $\{\hpi_{n_0,n_0'}\}_{n_0,n'_0\in\mathbb N}$ is tight; any weak limit point $\pi_\infty$ has marginals
$\mu_0$ and $\mu_0'$, and since
\[
\widehat\pi_{n_0,n_0'}\!\bigg(\bigg\{(z,z') : d'_{\f}\big(\f(z),z'\big)>\underset{\to 0}{\underbrace{{\rho(\widehat\nu_0^{(n_0)},\mh_0'^{(n_0')})}}}\bigg\}\bigg)\xrightarrow[]{n_0,n'_0\to\infty}0,
\]
we obtain $\pi_{n_0,n'_0}\stackrel w\longrightarrow\pi_\f$. 

Since the argument above was carried out for an arbitrary $\omega\in\Omega^\star$ and
$\mathbb P(\Omega^\star)=1$, we conclude that
\[
d'_{\phi^*_{n_0,n_0'}}\ \longrightarrow\ d'_{\f}\quad \mu_0'\!\otimes\!\mu_0'\text{-a.e.},\qquad
\widehat\pi^*_{n_0,n_0'}\ \stackrel{w}{\longrightarrow}\ \pi_{\f},
\]
almost surely as $n_0,n_0'\to\infty$. Hence the proof is complete.

\end{proof}

\subsection{Proof of Theorem  3.1}

\begin{proof}[Proof of Theorem 3.1]

Just like in the proof of Lemma 3.1, fix i.i.d.\ sequences 
$Z_0:=\{z_{0i}\}_{i\ge1}\sim\mu_0$, 
$Z_0':=\{z'_{0k}\}_{k\ge1}\sim\mu_0'$, 
and $Z_1:=\{z_{1j}\}_{j\ge1}\sim\mu_1$, all mutually independent, and let
\[
\widehat\mu_0^{(n_0)}:=\frac1{n_0}\sum_{i=1}^{n_0}\delta_{z_{0i}}, 
\qquad
\widehat\mu_0'^{(n_0')}:=\frac1{n_0'}\sum_{k=1}^{n_0'}\delta_{z'_{0k}},
\qquad
\widehat\mu_1^{(n_1)}:=\frac1{n_1}\sum_{j=1}^{n_1}\delta_{z_{1j}}
\]
denote the empirical measures formed from their first $n_0,n_0',n_1$ observations, respectively.
Since $\Z,\Z'$ are Polish, by Varadarajan’s theorem \citep[Theorem~11.4.1]{dudley2002real} there exists an event
\[
\Omega_{\mathrm{emp}}\in\mathcal F,\qquad \mathbb P(\Omega_{\mathrm{emp}})=1,
\]
such that on $\Omega_{\mathrm{emp}}$ we have simultaneously
\[
\widehat\mu_0^{(n_0)}\stackrel{w}{\longrightarrow}\mu_0,\qquad
\widehat\mu_0'^{(n_0')}\stackrel{w}{\longrightarrow}\mu_0',\qquad
\widehat\mu_1^{(n_1)}\stackrel{w}{\longrightarrow}\mu_1
\quad\text{as }n_0,n_0',n_1\to\infty.
\]

By the \cite{kuratowski1965selectors} measurable selection theorem, 
we can fix measurable selectors
\[
(\widehat\pi^*_{n_0,n_0'},\phi^*_{n_0,n_0'})\in
\arg\min_{\hpi\in\Pi(\widehat\mu_0^{(n_0)},\widehat\mu_0'^{(n_0')}),\ \phi\in\Phi}
\Big\{\mathscr L_{\FGW_\alpha}(\hpi,d'_\phi)+\lambda\,\mathscr L_G(\hpi,d'_\phi)\Big\},
\]
and, for each $z\in\Z$, 
\[
\widehat z'_{n_0,n_0'}(z)\in
\arg\min_{z'\in\Z'}\;
\mathscr L_S\!\big(z'\mid z,(\widehat\pi^*_{n_0,n_0'},\phi^*_{n_0,n_0'}),\lambda_S\big).
\]

Set $\Omega^\star:=\Omega_{\mathrm{emp}}$. 
In what follows we fix an arbitrary $\omega\in\Omega^\star$ and suppress the dependence on $\omega$; 
all limits are then deterministic along this sample path. Accordingly, by Lemma 3.1, along this sample path we have
\[
d'_{\phi^*_{n_0,n_0'}}\ \longrightarrow\ d'_{\f}
\quad\text{$\mu_0'\!\otimes\!\mu_0'$-a.e. on $\Z'\!\times\!\Z'$,}
\qquad
\widehat\pi^*_{n_0,n_0'}\ \stackrel{w}{\longrightarrow}\ \pi_\f,
\quad\text{as }n_0,n_0'\to\infty.
\]
For fixed $z\in\Z$, define the \emph{population objective}
\[
\mathscr L_S^{(\infty)}(z'\mid z)
:=\int_{\Z\times\Z'} \big|d_Z(u,z)-d'_{\f}(v,z')\big|\,d\pi_\f(u,v)
+\lambda_S\,d'_{\f}\!\big(z',\f(z)\big).
\]

As in the proof of Lemma 3.1, integration over the deterministic coupling $\pi_\f$ boils down to integration over the marginal $\mu_0$, yielding
\[\begin{aligned}
\mathscr L_S^\infty\big(z'\mid z\big)
&= \int_{\Z}\;\Big|d_Z(u,z)-d_Z(u,\f^{-1}(z'))\Big|d\mu_0(u) \;+\;\lambda_S d'_\f(z',\f(z))\;,
\end{aligned}
\]
which vanishes at $z'=\f(z)$, resulting in
$\mathscr L_S^\infty(\f(z)\mid z)=0$. Also for any $z'\neq \f(z)$ we have $\mathscr L_S^{(\infty)}(z'\mid z)\ge \lambda_S\,d'_{\f}(z',\f(z))>0$. Hence $\f(z)$ is the unique minimizer and, for every $\varepsilon>0$,
\begin{equation}\label{eq:strict-gap-thm}
\inf_{\{z':\,d'_{\f}(z',\f(z))\ge \varepsilon\}}
\mathscr L_S^{(\infty)}(z'\mid z)\ \ge\ \lambda_S\,\varepsilon\ >0.
\end{equation}

Now, for $z\in\Z$ and $z'\in\Z'$, write the \emph{sample objective}
\[
\mathscr L_S^{(n_0,n_0')}(z'\mid z)
:=\int_{\Z\times\Z'} \big|d_Z(u,z)-d'_{\phi^*_{n_0,n_0'}}(v,z')\big|\,d\widehat\pi^*_{n_0,n_0'}(u,v)
+\lambda_S\,d'_{\phi^*_{n_0,n_0'}}\!\big(z',\phi^*_{n_0,n_0'}(z)\big).
\]

Define
\[
G_{z,z'}(u,v):=\big|d_Z(u,z)-d'_{\f}(v,z')\big|,
\qquad
G^{(n_0,n_0')}_{z,z'}(u,v):=\big|d_Z(u,z)-d'_{\phi^*_{n_0,n_0'}}(v,z')\big|.
\] As in the proof of Lemma 3.1, without loss of generality (replacing a metric $d$ by a topologically equivalent bounded metric $\bar d(\cdot,\cdot):=\psi(d(\cdot,\cdot))$) assume $d_Z\in C_b(\Z\times \Z)$, hence both $G_{z,z'}, G_{z,z'}^{(n_0,n'_0)}$ are bounded as well $$G_{z,z'}, G_{z,z'}^{(n_0,n'_0)}\leq 2\|d_Z\|_{\infty}\;.$$
Working on $\omega\in \Omega^\star$, Lemma 3.1 gives
$\widehat\pi^*_{n_0,n_0'}\stackrel{w}{\longrightarrow}\pi_\f$
and $d'_{\phi^*_{n_0,n_0'}}\to d'_{\f}$ $\mu_0'\!\otimes\!\mu_0'$–a.e.
Choose $\varepsilon>0$. As in \eqref{eq:K^c}, by tightness of $\{\widehat\pi^*_{n_0,n_0'}\}$ and $\pi_\f$
(Prokhorov), we may pick a compact $K=K_1\times K_2\subset\Z\times\Z'$ with
\[
\sup_{n_0,n_0'}\widehat\pi^*_{n_0,n_0'}(K^\complement)\ \vee\ \pi_\f(K^\complement)\ <\ \varepsilon.
\]
By Lusin's theorem \citep[Theorem~7.1.13]{bogachev2007measureI}, there exists a compact $K'\subset\Z'$ with $\mu_0'(K')>1-\varepsilon$ such that
$\f^{-1}$ is continuous on $K'$, hence $d'_{\f}$ is continuous on $K'\times K'$.
Set $\widetilde K:=K_1\times(K_2\cap K')$.

On $\widetilde K$, the integrand $G_{z,z'}$ is continuous and bounded, and
$G^{(n_0,n_0')}_{z,z'}\to G_{z,z'}$ pointwise. Consequently, for any compact $C\subset K'$ we have
\[
\begin{aligned}
\sup_{z'\in C}\Big|
\!\int_{\widetilde K} G^{(n_0,n_0')}_{z,z'}\,d\widehat\pi^*_{n_0,n_0'}
-\!\int_{\widetilde K} G_{z,z'}\,d\pi_\f
\Big|
&\le
\underbrace{\sup_{z'\in C}\int_{\widetilde K}\!\big|G^{(n_0,n_0')}_{z,z'}-G_{z,z'}\big|\,d\widehat\pi^*_{n_0,n_0'}}_{(\mathrm{I})}\\
&\quad+\underbrace{\sup_{z'\in C}\Big|\!\int_{\widetilde K}\!G_{z,z'}\,d\widehat\pi^*_{n_0,n_0'}-\!\int_{\widetilde K}\!G_{z,z'}\,d\pi_\f\Big|}_{(\mathrm{II})}\\
&\quad + \varepsilon\,\sup_{z'\in C}\|G_{z,z'}\|_\infty
+ \varepsilon\,\sup_{z'\in C}\|G^{(n_0,n_0')}_{z,z'}\|_\infty.
\end{aligned}
\]

By Egorov's theorem, for any $\eta>0$ there exists a compact $E\subseteq \widetilde K$ with $\sup_{n_0,n_0'}\widehat\pi^*_{n_0,n_0'}(\widetilde K\setminus E)<\eta$ such that the convergence of $G_{z,z'}^{(n_0,n'_0)}$ becomes uniform \[
\sup_{(u,v)\in E}\big|G^{(n_0,n_0')}_{z,z'}(u,v)-G_{z,z'}(u,v)\big|\xrightarrow{n_0,n_0'\to\infty}0.
\]

Also, because $(u,v,z')\mapsto G_{z,z'}(u,v)$ is continuous on the compact set $E\times C$, the map
$z'\mapsto G_{z,z'}|_E$ is continuous from $C$ into $(C_b(E),\|\cdot\|_\infty)$. Hence, the family
\[
\mathcal G_C\; :=\; \big\{\,G_{z,z'}\big|_E:\; z'\in C\,\big\}\; \subseteq\; C_b(E)
\]
is the continuous image of a compact set and is therefore compact in $\big(C_b(E),\|\cdot\|_\infty\big)$. Therefore, $\mathcal G_C$ is a compact metric space, and thus is totally bounded, meaning for every $\delta>0$
there exist finitely many $z'_1,\dots,z'_m\in C$ with $G^{(r)}:=G_{z,z'_r}\big|_E$ such that
\[
\mathcal G_C\; \subset\; \bigcup_{r=1}^m B_\infty\!\big(G^{(r)},\delta\big),\]
\noindent where $B_\infty(f,\delta):=\{g\in C_b(E):\; \|g-f\|_\infty<\delta\}$ are open balls in $\big(C_b(E),\|\cdot\|_\infty\big)$.

By Egorov’s theorem, for each $r=1,\dots,m$ there exists a compact $E_r\subset\widetilde K$ (chosen above) such that
\[
\sup_{(u,v)\in E_r}\big|G^{(n_0,n_0')}_{z,z'_r}(u,v)-G_{z,z'_r}(u,v)\big|\xrightarrow[]{n_0,n_0'\to\infty}0.
\] Replace $E$ by the compact set of finite intersections $$\bigcap_{r=1}^m E_r \;\;\cap E\;. $$
Now, for any $z'\in C$ choose $r$ with $\|G_{z,z'}|_E-G_{z,z'_r}|_E\|_\infty<\delta$; then
\[
\begin{aligned}
\sup_{(u,v)\in E}\big|G^{(n_0,n_0')}_{z,z'}-G_{z,z'}\big|
&\le \sup_{E}\big|G^{(n_0,n_0')}_{z,z'}-G^{(n_0,n_0')}_{z,z'_r}\big|
+\sup_{E}\big|G^{(n_0,n_0')}_{z,z'_r}-G_{z,z'_r}\big|
+\sup_{E}\big|G_{z,z'_r}-G_{z,z'}\big|\\
&\le 2\delta+\sup_{E}\big|G^{(n_0,n_0')}_{z,z'_r}-G_{z,z'_r}\big|.
\end{aligned}
\]
Taking $\sup_{z'\in C}$ and letting $n_0,n_0'\to\infty$, $\delta\downarrow0$, yields
\[
\sup_{z'\in C}\ \sup_{(u,v)\in E}\big|G^{(n_0,n_0')}_{z,z'}-G_{z,z'}\big|\ \longrightarrow\ 0.
\]

Accordingly, for $(\mathrm I)$ we have
\[
\begin{aligned}
\sup_{z'\in C}\int_{\widetilde K}\!\big|G^{(n_0,n_0')}_{z,z'}-G_{z,z'}\big|\,d\widehat\pi^*_{n_0,n_0'}
&\le\;
\sup_{z'\in C}\ \sup_{(u,v)\in E}\big|G^{(n_0,n_0')}_{z,z'}-G_{z,z'}\big|\\
&\qquad+\; 2\|d_Z\|_\infty\cdot \widehat\pi^*_{n_0,n_0'}(\widetilde K\setminus E)\\
&\xrightarrow[\eta\downarrow 0]{\; n_0,n'_0\to\infty\; } 0,
\end{aligned}
\]
so $(\mathrm I)\to0$ as $n_0,n_0'\to\infty$.

Similarly, for $(\mathrm{II})$, take the finite covering $\bigcup_{r=1}^m B_\infty(G^{(r)},\delta)$ of $\mathcal G_C$. Since $\widehat\pi^*_{n_0,n_0'}\xrightarrow[]{w}\pi_\f$ and $E$ is compact, the Portmanteau theorem
\cite[Thm.\ 2.1]{billingsley1999convergence} gives, 
\[\int_E G^{(r)}\,d\widehat\pi^*_{n_0,n_0'}\to\int_E G^{(r)}\,d\pi_\f,\quad \foral r\in 1,\dots, m\;.\]
Now, for any $F\in\mathcal G_C$ choose $r$ with $\|F-G^{(r)}\|_\infty<\delta$; then
\[
\Big|\!\int_E F\,d\widehat\pi^*_{n_0,n_0'}-\!\int_E F\,d\pi_\f\Big|
\ \le\ \delta\;+\;\Big|\!\int_E G^{(r)}\,d\widehat\pi^*_{n_0,n_0'}-\!\int_E G^{(r)}\,d\pi_\f\Big|\;+\;\delta.
\]
Taking $\sup_{F\in\mathcal G_C}$ and noting the middle term is a {finite} maximum over $r=1,\dots,m$,
\[
\sup_{F\in\mathcal G_C}\Big|\int_E F\,d\widehat\pi^*_{n_0,n_0'}-\int_E F\,d\pi_\f\Big|
\ \le\ 2\delta\;+\;\max_{1\le r\le m}\Big|\int_E G^{(r)}\,d\widehat\pi^*_{n_0,n_0'}-\int_E G^{(r)}\,d\pi_\f\Big|
\ \xrightarrow[n_0,n_0'\to\infty]{}\ 2\delta,
\]
 and taking $\delta\downarrow0$
\[
\sup_{z'\in C}\Big|\int_{\widetilde K}G_{z,z'}\,d\widehat\pi^*_{n_0,n_0'}-\int_{\widetilde K}G_{z,z'}\,d\pi_\f\Big|\ \longrightarrow\ 0.
\]
Thus $(\mathrm{II})\to 0$ uniformly over $z'\in C$. Having $\varepsilon\downarrow 0$ thus yields 

\begin{equation}
    \label{eq: G_uniconv}
    \sup_{z'\in C}\Big|
\!\int_{\widetilde K} G^{(n_0,n_0')}_{z,z'}\,d\widehat\pi^*_{n_0,n_0'}
-\!\int_{\widetilde K} G_{z,z'}\,d\pi_\f
\Big|\xrightarrow[]{n_0,n'_0\to \infty}0 \quad \text{for }\mu_0-\text{a.e. }z\in\Z
\end{equation}

Next, for the penalty term $\lambda_S\,d'_{\phi^*_{n_0,n_0'}}(z',\phi^*_{n_0,n_0'}(z))$, use the identity
\[
d'_{\phi}(z',\phi(z)) \;=\; d_Z\!\big(\phi^{-1}(z'),\, z\big),\qquad
d'_{\f}(z',\f(z)) \;=\; d_Z\!\big(\f^{-1}(z'),\, z\big).
\]
By Lemma 3.1 and $\f_{\#}\mu_0=\mu_0'$, we have $\phi^*_{n_0,n_0'}(z)\to \f(z)$ for $\mu_0$–a.e.\ $z$, which implies (by change of variables and bijectivity) $\phi_{n_0,n_0'}^{-1}(z')\to \f^{-1}(z')$ for $\mu_0'$–a.e.\ $z'$. 
Applying Egorov's theorem on $\Z'$ yields, for any $\eta>0$, a compact $D\subset \Z'$ with $\mu_0'(D)>1-\eta$ such that $\phi_{n_0,n_0'}^{-1}\to \f^{-1}$ \emph{uniformly} on $D$. Since $d_Z(\cdot,z)$ is continuous, for $\mu_0$–a.e.\ fixed $z$ and any compact neighborhood $C$ of $\f(z)$ we have
\[
\sup_{z'\in C}\big|d_Z(\phi_{n_0,n_0'}^{-1}(z'),z)-d_Z(\f^{-1}(z'),z)\big|\; \longrightarrow\; 0.
\]
Equivalently,
\begin{equation}\label{eq:lambda_d_uniconv}
\sup_{z'\in C}\big|\lambda_S\,d'_{\phi^*_{n_0,n_0'}}(z',\phi^*_{n_0,n_0'}(z))
-\lambda_S\,d'_\f(z',\f(z))\big|\xrightarrow[n_0,n_0'\to\infty]{}0,
\quad \text{for $\mu_0$–a.e.\ $z\in\Z$.}
\end{equation}

Combining \eqref{eq: G_uniconv} and \eqref{eq:lambda_d_uniconv} gives, for $\mu_0$–a.e.\ fixed $z$ and any compact neighborhood $C$ of $\f(z)$,
\begin{equation}
\label{eq: L_S_uniconv}
\sup_{z'\in C}\Big|\mathscr L_S^{(n_0,n_0')}(z'\mid z) - \mathscr L_S^{(\infty)}(z'\mid z)\Big|\ \longrightarrow\ 0.
\end{equation}

Observe that $\mathscr L_S^{(n_0,n_0')}(z\!'\mid z), \mathscr L_S^{(\infty)}(z'\mid z)$ are both proper and lower semi-continuous, and for any $c\in\R$ the level set for $\mathscr L_S^{(n_0,n_0')}(\cdot\mid z)$ is contained in a closed ball of finite radius:
$$\Bigl\{z'\in\Z': \mathscr L_S^{(n_0,n_0')}(z\!'\mid z)\leq c\Bigr\}\subseteq \Bigl\{z'\in\Z':  d'_{\phi^*_{n_0,n_0'}}\!\big(z',\phi^*_{n_0,n_0'}(z)\big)
\le c/\lambda_S\Bigr\}\;,$$
thus $\mathscr L_S^{(n_0,n_0')}( \cdot \mid z)$ is eventually level–bounded. 

The above conditions, together with the strict local gap \eqref{eq:strict-gap-thm} and uniform convergence on compact neighborhoods \eqref{eq: L_S_uniconv} imply \emph{epi–convergence} \cite[Prop.\ 7.2 and Thm.\ 7.17]{rockafellar1998variational}:

\[
\mathscr L_S^{(n_0,n_0')}( \cdot \mid z)\ \xrightarrow{\,e\,}\ \mathscr L_S^{(\infty)}(\cdot \mid z),
\]

And epi-convergence in turn implies \emph{argmin convergence}
\cite[Theorem~7.31--7.33]{rockafellar1998variational}. Hence, the argmin sets of
$\mathscr L_S^{(n_0,n_0')}( \cdot \mid z)$ are eventually nonempty and bounded and satisfy
\[
\limsup_{n_0,n_0'\to\infty}\;\arg\min_{z'}\mathscr L_S^{(n_0,n_0')}(z'\mid z)
\; \subseteq\; \arg\min_{z'}\mathscr L_S^{(\infty)}(z'\mid z)=\{\f(z)\}.
\]
Because the limit argmin is a singleton, every choice

\vspace{2.5mm}

\centerline{$\displaystyle\widehat z'_{n_0,n_0'}(z)\in \arg\min_{z'\in\Z'}\mathscr L_S^{(n_0,n_0')}(z'\mid z)$}

\vspace{2.5mm}

converges to $\f(z)$; equivalently,

\vspace{2.5mm}

\centerline{$\displaystyle
d'_{\f}\!\big(\widehat z'_{n_0,n_0'}(z),\,\f(z)\big)\; \longrightarrow\; 0\;,$}

\vspace{2.5mm}

for $\mu_0$–a.e.\ $z$.

Now, let
\(
A\;:=\;\Bigl\{z\in\Z:\ d'_{\f}\!\big(\widehat z'_{n_0,n_0'}(z),\,\f(z)\big)\ \longrightarrow\ 0\Bigr\}.
\) Assumption 3.3 yields absolute continuity of the treatment distribution, \(\mu_1\ll\mu_0\). 
Hence, $\mu_0(A^\complement)=0$ implies $\mu_1(A^\complement) =0$, and
\begin{equation}\label{eq:argmin_conv}
d'_{\f}\!\big(\widehat z'_{n_0,n_0'}(z),\,\f(z)\big)\;\longrightarrow\;0
\qquad\text{for $\mu_1$–a.e.\ }z\in\Z.
\end{equation}

Next, fix $f\in C_b(\Z')$. For $z\in\Z$ set $g_{n_0,n_0'}(z):=f\!\big(\widehat z'_{n_0,n_0'}(z)\big)$ and
$g(z):=f\!\big(\f(z)\big)$. By the previous display, $g_{n_0,n_0'}(z)\to g(z)$ for $\mu_1$–a.e.\ $z$, and
$|g_{n_0,n_0'}(z)|\le\|f\|_\infty$. Hence, by dominated convergence,
\[
\int g_{n_0,n_0'}\,d\mu_1\ \longrightarrow\ \int g\,d\mu_1=\int f\,d(\f_{\#}\mu_1)=\int f\,d\mu_1'.
\]
Now fix $n_1\in\mathbb N$. On $\Omega^\star$ we have $\{z_{1j}\}_{j\ge1}\sim\mu_1$ i.i.d.\ and
$z_{1j}\in A$ for all $j$ where $A\subset\Z$ is a full–$\mu_1$ set on which the pointwise
convergence above holds. Therefore, for each fixed $n_1$,
\[
\frac1{n_1}\sum_{j=1}^{n_1} f\!\big(\widehat z'_{n_0,n_0'}(z_{1j})\big)
\ \xrightarrow[n_0,n_0'\to\infty]{}\ 
\frac1{n_1}\sum_{j=1}^{n_1} f\!\big(\f(z_{1j})\big).
\]
Letting $n_1\to\infty$ and applying the strong law to $f\circ\f$ yields
\[
\frac1{n_1}\sum_{j=1}^{n_1} f\!\big(\f(z_{1j})\big)\ \longrightarrow\ \int f\,d\mu_1'.
\]
A diagonal argument in $(n_0,n_0')$ and $n_1$ gives
\[
\frac1{n_1}\sum_{j=1}^{n_1} f\!\big(\widehat z'_{n_0,n_0'}(z_{1j})\big)\ \longrightarrow\ \int f\,d\mu_1',
\qquad\text{as }n_0,n_0'\to\infty,\ n_1\to\infty,
\]
that is, $\widehat\mu_1'\ \stackrel{w}{\longrightarrow}\ \mu_1'$ on $\Omega^\star$.
Since $f\in C_b(\Z')$ was arbitrary, the proof is complete.

\end{proof}

\section{Simulation and Baseline Details}

This section provides a detailed description of the simulation setup, including the data-generating processes, effect modification mechanisms, and parameter choices. Additionally, we outline the baseline models used for comparison, detailing their implementation and adaptation to our specific problem setting.

\subsection{Data Generation and Parameters}\label{app:simulation_details}

We generate covariate vectors $\mathbf{x}_i \in \mathbb{R}^{d}$ independently from a multivariate normal distribution
\[
x_{ik} \stackrel{\text{i.i.d.}}{\sim} \mathcal N(2.5,\, 1.5), \qquad k=1,\dots,d,
\]
and augment with an intercept to form $x_i = [1,\,x_{i1},\dots, x_{id}]^\top$.  
Each observation receives a binary treatment assignment $D_i\in\{0,1\}$ and produces the response
\[
y_i = \alpha + x_i^\top \beta + D_i\cdot(\tau + x_i^\top \gamma) + \varepsilon_i,\qquad 
\varepsilon_i \stackrel{\text{i.i.d.}}{\sim} \mathcal N(0,\,1.5),
\]
where $\beta,\gamma\in\mathbb{R}^{d+1}$ are randomly drawn from $\text{Uniform}(-1,1)$ and rescaled to satisfy
$\|\beta\|_2^2=2$ and $\|\gamma\|_2^2=1.5$.  
The treatment effect baseline is fixed at $\tau=10$.  
Samples with $D_i=0$ and $D_i=1$ define the source control and treatment sets $Z_0$ and $Z_1$ respectively,
with each observation $z_i=(x_i,y_i)\in\mathbb{R}^{d+1}$.

Cross-site heterogeneity is generated via a map $\f:\mathbb{R}^{d+1}\!\to\!\mathbb{R}^{d+1}$,
applied independently to subsets of $(Z_0,Z_1)$ to create the target-site datasets $(Z_0',Z_1')$.
We construct a lower–triangular mixing matrix $\Omega\in\mathbb{R}^{(d+1)\times(d+1)}$ whose rows sum to one:
\[\begin{cases}
\Omega_{11}=1,\\ \Omega_{21}=-\tfrac{2}{3},\quad
\Omega_{22}=1-\Omega_{21},\\
\Omega_{ij}=-\tfrac{1}{2}(0.6)^{\,i-j-1}\ \text{for } j<i,
\quad
\Omega_{ii}=1-\sum_{j<i}\Omega_{ij},\qquad \text{for }\ i\ge2;\end{cases}
\] So for instance:
$$\Omega_{(d=2)}=\begin{bmatrix}
  1 & 0 & 0 \\
 -0.667 & 1.667 & 0 \\
 -0.5 & -0.3 & 1.8
\end{bmatrix}\;,\qquad \Omega_{(d=3)}=\size{.8}{\begin{bmatrix}
  1 & 0 & 0 & 0 & 0  \\
 -0.667 & 1.667 & 0 & 0 & 0  \\
 -0.5 & -0.3 & 1.8 & 0 & 0  \\
 -0.5 & -0.3 & -0.18 & 1.98 & 0  \\
 -0.5 & -0.3 & -0.18 & -0.108 & 2.088 
\end{bmatrix}}\;.$$
The site map is always $\f(z)=\Omega^\top\psi(z)+b$ for a fixed offset $b=[3,3,\dots,3]\in\mathbb{R}^{d+1}$.

\subsubsection{Scenario-specific transformations}

Each scenario defines a transformation $\psi$ describing how $(Z_0,Z_1)$ are mapped to $(Z_0',Z_1')$.
Unless otherwise stated, the feature dimensionality is $d=2$ and treatment assignment is randomized.

The baseline setting (\emph{Scenario 1}) uses the linear site map
\[
\psi(z)=z,\qquad \f(z)=\Omega_1^\top z + b,
\]
corresponding to an ideal randomized trial with perfect covariate overlap.

To introduce smooth curvature (\emph{Scenario 2}), we define
\[
\psi(z)=
\begin{bmatrix}
x + 0.2\,\tanh(x^{\circlearrowleft})\\[2pt]
y + 0.15\,\tanh(0.3\,\|x\|_2^2)
\end{bmatrix},
\qquad 
x^{\circlearrowleft}=(x_2,\ldots,x_d,x_1),
\]
so that $\psi$ applies a cyclic coordinate shift to $x$ and a $\tanh$–based nonlinear adjustment to $y$.
  
The stronger nonlinearity (\emph{Scenario 3}) is implemented with heterogeneous feature scaling
and a sinusoidal bending of the response dimension:
\[
\psi(z)=
\begin{bmatrix}
x\odot(1+\alpha)\\[2pt]
y + R\sin\theta
\end{bmatrix},
\qquad
\alpha_j = 0.15\,\frac{j - \frac{d-1}{2}}{\max\{\frac{d-1}{2},10^{-12}\}},
\]
\[
\theta = \frac{\pi}{2}\!\left(1+\tanh\!\frac{y-\mathbb{E}[y]}{\operatorname{sd}(y)+10^{-12}}\!\right),\qquad
R = 0.6\,Q_{0.75}(\|x\|_2) + 10^{-12}.
\]
 
To generate sharp, discontinuous regime changes (\emph{Scenario 4}), we define a discontinuous map
\[
\psi(z)=
\begin{bmatrix}
x + \1_{\{x_1>2.5\}}\mathbf{1}_d\\[2pt]
y
\end{bmatrix},
\]
which adds $1$ to all feature coordinates if the first covariate exceeds $2.5$.  
This non-bijective transformation produces bimodality and cluster separation in the target site.

For the non-RCT setting (\emph{Scenario 5}), treatment assignment is no longer randomized.
Instead, the covariate means depend on treatment status:
\[
X_i\mid D_i \sim \mathcal N_d(\mu_x + \kappa D_i,\; \sigma_x^2 \mathcal I_d),\quad \kappa = 3\;.
\]
thereby inducing systematic imbalance between treatment and control units.
  
Lastly, \emph{Scenario 6} replicates the affine transformation of \emph{Scenario 1} with feature dimension $d=30$,
allowing assessment of scalability and robustness to dimensionality.

\subsubsection{Additional robustness scenarios}
Several further transformations are used to evaluate robustness under complex nonlinearities.

\smallskip
\emph{7- Radial:}
\[
\psi(z)=
\begin{bmatrix}
x\,s(r)\\[2pt]
y + 0.24\,r
\end{bmatrix},
\qquad 
s(r)=1+0.32\,\tanh(0.6r)+0.05\,\tanh(0.12r^2),\quad r=\|x\|_2.
\]
This map performs radial scaling of the features with mild coupling into $y$.

\smallskip
\emph{8- Curvy:}
\[
\psi(z)=
\begin{bmatrix}
x + a_1\sin(b_1x)+a_2\sin(b_2xP)+a_3\tanh(c r)\tfrac{x}{r+10^{-8}}\\[2pt]
y + d_1\tanh(e r^2)+d_2\sin(f\,x^\top u)
\end{bmatrix},
\]
where $P$ is a random orthogonal matrix, $u$ a random unit vector, and $r=\|x\|_2$.
Constants are fixed at 
$a_1{=}0.35$, $a_2{=}0.25$, $a_3{=}0.20$, $b_1{=}0.9$, $b_2{=}1.4$, 
$c{=}0.6$, $d_1{=}0.45$, $d_2{=}0.25$, $e{=}0.15$, and $f{=}1.1$.

\smallskip
\emph{9- Smooth nonlinear, nonRCT:}
Combining the smooth map of \emph{Scenario~2} with covariate mean shift of \emph{Scenario 5}.

\smallskip
\emph{10- Smooth nonlinear, $d{=}30$:}
Combining the smooth map of \emph{Scenario~2} with higher-dimensional covariates, $d=30$.

\smallskip
\emph{11- Linear, $d{=}30$, nonRCT:}
linear map $\psi(z)=z$ with both high-dimensionality and nonrandomized treatment assignment.

For a visualization of how each scenario transforms a reference planar surface in $\R^{d+1}$, see the bottom row of Figure~\ref{fig: additional_scenarios}.

\subsection{Baseline Model Descriptions} \label{app:baseline_details}

The Two-way Fixed Effects  (\model{TWFE}) baseline is a straightforward extension of linear regression that accounts for treatment effects and target-specific effects by introducing distinct linear effects associated with belonging to the treatment group, $D_i=\1_{z\in Z_1\text{ or }Z'_1}$, and the target site, $T_i=\1_{z\in Z'_0\text{ or }Z'_1}$. These effects are estimated through a unified regression across the observed datasets $Z_0,Z_1,Z'_0$ minimizing the squared residuals:
    $$[\widehat\alpha,\widehat\beta,\widehat\tau,\widehat\gamma,\widehat\nu,\widehat\lambda] = \argmin_{[\alpha,\beta,\tau,\gamma,\nu,\lambda]} \sum_{Z_0,Z_1,Z'_1}\bigg(y_i - \big(\alpha + \mathbf{x}_i^\top\cdot\beta + D_i\cdot(\tau + \mathbf{x}_i^\top\cdot\gamma) + T_i\cdot (\nu + \mathbf{x}_i^\top\cdot\lambda)\big)\bigg)^2.$$
    
    Using the estimated parameters, the model generates synthetic responses for the target treatment group based on the target control data:
    $$y_{1i}^{\text{synth}} = \widehat\alpha + {\mathbf{x}'}_{0i}^\top\cdot\widehat\beta + (\widehat\tau + {\mathbf{x}'}_{0i}^\top\cdot\widehat\gamma) +  (\widehat\nu + {\mathbf{x}'}_{0i}^\top\cdot\widehat\lambda)\qqq \text{ for each }[{\mathbf{x}'}_{0i},y'_{0i}]\in Z'_0.$$

Inspired by the work of \cite{hotz2005predicting}, the \model{MatchSynth} baseline begins by identifying, for each control data point in the target dataset, a match from the source treatment dataset that minimizes the feature distance: $$z^{\text{m}}_{1i} = \argmin_{z_1=[x_{1},y_1]\in Z_1}\|x_1 - x'_{0i}\|_2\qqq\text{ for each }[x'_{0i},y'_{0i}]\in Z'_0,$$
thereby constructing the matched treatment dataset, $Z_1^\text{m}$. The matched outcomes are then regressed on the covariates to adjust for potential biases in the matches and compute the synthetic responses: \begin{align*}[\widehat\alpha, \widehat\beta] &= \argmin_{[\alpha,\beta]}\sum_{Z_1^{\text{m}}}\bigg(y_{1i}^{\text{m}} - \big(\alpha+ {\mathbf{x}_{1i}^\text{m}}^\top\cdot\beta\big)\bigg)^2;\\y_{1i}^{\text{synth}} &= y_{1i}^\text{m} + \widehat\beta\cdot(x'_{0i}-x_{1i}^\text{m})\qqq \text{ for each } z_{0i}'=[{\mathbf{x}'}_{0i},y'_{0i}]\in Z'_0 .\end{align*}

The \model{GenSynth} baseline combines the \model{MatchSynth} approach with the Generalized Synthetic Control framework \citep{xu2017generalized}. Accordingly, it begins by matching each source control and treatment observations with an observation in the target control dataset: \begin{align*}
    {z'}^{\text{m}}_{0i} &= \argmin_{z'_0=[x'_{0},y'_0]\in Z_0'}\|x_0' - x_{0i}\|_2\qqq\text{ for each }z_{0i}=[x_{0i},y_{0i}]\in Z_0,&\text{ and}\\
    {z'}^{\text{m}}_{1i} &= \argmin_{z'_0=[x'_{0},y'_0]\in Z_0'}\|x_0' - x_{1i}\|_2\qqq\text{ for each }z_{1i}=[x_{1i},y_{1i}]\in Z_1,
\end{align*} thereby constructing datasets $Z_0^\text{m}$ and $Z_1^\text{m}$. Next, it assumes common factors $F= [f,f']^\top$ for belonging to the source dataset, $f=[f_1,\dots,f_r]^\top$ and the target dataset $f'=[f'_1,\dots,f'_r]^\top$ and for each pairs constructs the following linear factors model: \begin{align*}&\begin{cases}
    y_{0i} &= \alpha + \mathbf{x}_{0i}^\top\cdot \beta + \lambda_{0i}^\top\cdot f + \epsilon_{0i}\\ {y'}_{0i}^\text{m} &= \alpha + {{\mathbf{x}'}_{0i}^\text{m}}^\top\cdot \beta + \lambda_{0i}^\top \cdot f' + \epsilon_{0i}'\end{cases} &\text{ for any }z_{0i}\in Z_0\text{ , and the matched }{z'}_{0i}^\text{m}&\ \text{, and}\\
    &\begin{cases}
    y_{1i} &= \alpha + \mathbf{x}_{1i}^\top\cdot \beta + \lambda_{1i}^\top\cdot f + \tau + \epsilon_{1i}\\ {y'}_{1i}^\text{m} &= \alpha + {{\mathbf{x}'}_{1i}^\text{m}}^\top\cdot \beta + \lambda_{1i}^\top \cdot f' + \epsilon_{1i}'\end{cases} &\text{ for any }z_{1i}\in Z_1\text{ , and the matched }{z'}_{1i}^\text{m}.
\end{align*}

where the estimation of parameters and synthetic responses will be done according to the following step by step computation:
\begin{align*}
    [ \widehat\alpha,\widehat\beta, \widehat F, \widehat\Lambda_0] &= \argmin_{[ \alpha,\beta,  F, \Lambda_0]} \sum_{z_{0i}\in Z_0} \left\| \begin{bmatrix}y_{0i}\\ {y'}_{0i}^\text{m}\end{bmatrix} - \begin{bmatrix}\alpha& +& {\mathbf{x}}_{0i}^\top\cdot \beta &+ \lambda_{0i}^\top \cdot f\\ \alpha& +& {{\mathbf{x}'}_{0i}^\text{m}}^\top\cdot \beta &+ \lambda_{0i}^\top \cdot f'\end{bmatrix} \right\|_2^2\\
    [ \widehat\Lambda_1, \widehat\tau] &= \argmin_{[ \Lambda_1, \tau]}\sum_{z_{1i}\in Z_1}\bigg(y_{1i} - \big(\widehat\alpha+\mathbf{x}_{1i}^\top\cdot \widehat\beta+\lambda_{1i}^\top\cdot \widehat f+\tau\big)\bigg)^2\\ 
    y_{1i}^{\text{synth}} &= y_{1i} + \widehat\beta\cdot\left(\mathbf{x}_{1i}^m - \mathbf{x}_{1i}\right) + \widehat\lambda_{1i}^\top\cdot (\widehat f - \widehat f')
\end{align*}

The \model{GANSynth} baseline adapts the CycleGAN framework \citep{zhu2017unpaired} to learn a mapping between the source and target control datasets ($Z_0$ and $Z'_0$). The model consists of two generator networks, $\Gamma:\mathcal{Z} \to \mathcal{Z}'$ and $\Phi:\mathcal{Z}' \to \mathcal{Z}$, which learn mappings from the source control dataset, $Z_0$, to the target control dataset, $Z'_0$, and vice versa. Additionally, two discriminators, $D_\Gamma$ and $D_\Phi$, are trained to distinguish between real and generated samples.

The discriminator $D_\Gamma$ is trained to maximize the adversarial loss between $D_\Gamma$ and $G$: $$\mathcal{L}_{\text{adv}}(D_\Gamma, \Gamma) = \mathbb{E}_{z' \sim Z'_0} [\log D_\Gamma(z')] + \mathbb{E}_{z \sim Z_0} [\log (1 - D_\Gamma(\Gamma(z)))],$$ while the generator $\Gamma$ is trained to minimize it, creating an adversarial game between the two networks. Same process applies to $D_\Phi$ and $\Phi$ with their corresponding adversarial loss:
\centermath{\mathcal{L}_{\text{adv}}(D_\Phi, \Phi) = \mathbb{E}_{z \sim Z_0} [\log D_\Phi(z)] + \mathbb{E}_{z' \sim Z'_0} [\log (1 - D_\Phi(\Phi(z')))].}
Additionally, a cycle consistency loss ensures that transforming a sample from source to target and back reconstructs the original input:

\vspace{2.5mm}

    \centerline{$\displaystyle \mathcal{L}_{\text{cycle}}(\Gamma, \Phi) = \mathbb{E}_{z \sim Z_0} \left[ \| \Phi(\Gamma(z)) - z \|_2^2 \right] + \mathbb{E}_{z' \sim Z'_0} \left[ \| \Gamma(\Phi(z')) - z' \|_2^2 \right].$}
    
\vspace{2.5mm}

The full optimization objective for the generators combines the adversarial and cycle consistency losses:
\centermath{\begin{aligned}
    \mathcal{L}(\Gamma, \Phi, D_\Gamma, D_\Phi) &= \mathcal{L}_{\text{adv}}(D_\Gamma, \Gamma) + \mathcal{L}_{\text{adv}}(D_\Phi, \Phi) + \lambda\cdot \mathcal{L}_{\text{cycle}}(\Gamma, \Phi).
\end{aligned}}
 Once trained, the generator $\Gamma$ is applied to the source treatment dataset $Z_1$ to produce the synthetic target treatment dataset: \centermath{{Z_1'}^{\text{synth}}=\Gamma(Z_1).}

\subsection{Evaluation metrics}\label{app:evaluation_metrics}

Each method produces a synthetic target--site treatment sample 
$Z'_1{}^{(\mathrm{synth})}$ consisting of joint observations 
$z'_i=(x'_i,y'_i)\in\mathbb{R}^{d+1}$. 
Performance is evaluated by comparing the synthesized sample to the oracle target sample 
$Z'_1$ along both marginal and joint dimensions.
\subsubsection{Marginal metrics for $Y$}
For the outcome variable $Y$, we report summary statistics
\centermath{\text{Mean},\quad \text{Std.\,dev},\quad q_1(25\%),\ q_2(\text{median}),\ q_3(75\%),}
together with several one–dimensional distributional distances between
the true and synthesized outcomes 
$Y'_1$ and $Y'_1{}^{(\mathrm{synth})}$.
Let $$P_{Y'_1}\;=\;\tfrac1{\left|Z'_1\right|}\sum_{i: z'_i\in Z'_1}\delta_{y_i'}\;,\qquad P_{Y'_1}^{(\mathrm{synth})}\;=\;\tfrac1{\left|Z'_1{}^{(\mathrm{synth})}\right|}\cdot\sum_{i: z'_i\in Z'_1{}^{(\mathrm{synth})}}\delta_{y_i'}\;,$$ denote the empirical distributions of the oracle and synthesized outcomes, respectively, 
with corresponding densities $p_{Y'_1}$ and $p_{Y'_1}^{(\mathrm{synth})}$.
We compute the following distances:
\begin{itemize}
\item {Wasserstein distance:}
  \[
  \W_1(P_{Y'_1}, P_{Y'_1}^{(\mathrm{synth})})
  ~=~
  \inf_{\pi\in\Pi(P_{Y'_1}, P_{Y'_1}^{(\mathrm{synth})})}
  \int_{\mathbb{R}\times\mathbb{R}}\!|y-y'|\,d\pi(y,y').
  \]

  \item {Total variation:}
  \[
  \tfrac{1}{2}\!\int_{\mathbb{R}}\!|p_{Y'_1}(y)-p_{Y'_1}^{(\mathrm{synth})}(y)|\,dy.
  \]

  \item {Hellinger distance:}
  \[
  \Big[\tfrac{1}{2}\!\int_{\mathbb{R}}\!\left(\sqrt{p_{Y'_1}(y)}-\sqrt{p_{Y'_1}^{(\mathrm{synth})}(y)}\right)^2\,dy\Big]^{1/2}.
  \]

  \item {Kullback–Leibler divergence:}
  \[
  \int_{\mathbb{R}} p_{Y'_1}(y)\cdot
  \log\!\Big(\frac{p_{Y'_1}(y)}{p_{Y'_1}^{(\mathrm{synth})}(y)}\Big)\,dy.
  \]
\end{itemize}

\subsubsection{Joint metrics for $Z=(X,Y)$}
To evaluate the fidelity of the joint distribution, we compare the oracle and synthesized samples,
$Z'_1$ and $Z'_1{}^{(\mathrm{synth})}$, using several multivariate metrics. 
Let
\[
P_{Z'_1} \;=\; \tfrac1{|Z'_1|}\!\sum_{i:\,z'_i\in Z'_1}\!\delta_{z'_i},
\qquad
P_{Z'_1{}^{(\mathrm{synth})}} \;=\; \tfrac1{|Z'_1{}^{(\mathrm{synth})}|}
\!\sum_{i:\,z'_i\in Z'_1{}^{(\mathrm{synth})}}\!\delta_{z'_i},
\]
denote the corresponding empirical distributions. We compute the following distances:

\begin{itemize}

\item {Energy distance:}
\[
E^2(Z'_1{}^{(\mathrm{synth})},Z'_1)
~=~
2\,\E_{\size{.7}{\overset{\displaystyle z\sim P_{Z'_1{}^{(\mathrm{synth})}}}{\displaystyle \!\!\!\!\!\!\!\!\!\!\!z'\sim  P_{Z'_1}}}}\!\|z-z'\|
~-~
\E_{z,z'\sim P_{Z'_1}}\!\|z-z'\|
~-~
\E_{z,z'\sim P_{Z'_1{}^{(\mathrm{synth})}}}\!\|z-z'\|.
\]

\item {Sliced Wasserstein distance:}
\[
\mathbb{SW}_1(Z'_1{}^{(\mathrm{synth})},Z'_1)
~=~
\frac{1}{K}\sum_{k=1}^{K} 
\W_1\!\big(
\langle v_k,Z'_1{}^{(\mathrm{synth})}\rangle,
\langle v_k,Z'_1\rangle
\big),
\qquad K=128,
\] where $v_k\!\sim\!\mathcal N(0,I_{d+1})$ are $K$ independent random directions in $\R^{d+1}$, and 
$\langle v_k, z\rangle$ denote the scalar projection of $z$ onto $v_k$.

\item {Projected divergences:}
\[
\mathrm{Proj\!-\!Div}(Z'_1{}^{(\mathrm{synth})},Z'_1)
~=~
\frac{1}{K}\sum_{k=1}^{K}
D\!\big(
\langle v_k,Z'_1{}^{(\mathrm{synth})}\rangle,
\langle v_k,Z'_1\rangle
\big),
\] where $D$ denotes any of the Total Variation, Hellinger, and 
Kullback–Leibler divergences, and each divergence is first evaluated in one dimension and then averaged over 
$K=128$ random projections onto $v_k\!\sim\!\mathcal N(0,I_{d+1})$.

\item {Maximum Mean Discrepancy (MMD) with Gaussian kernel:} \[
\mathrm{MMD}^2(Z'_1{}^{(\mathrm{synth})},Z'_1)
~=~
\E_{z,z'\sim P_{Z'_1}}[k(z,z')]
~+~
\E_{z,z'\sim P_{Z'_1{}^{(\mathrm{synth})}}}[k(z,z')]
~-~
2\,\E_{\size{.7}{\overset{\displaystyle z\sim P_{Z'_1{}^{(\mathrm{synth})}}}{\displaystyle \!\!\!\!\!\!\!\!\!\!\!z'\sim  P_{Z'_1}}}}[k(z,z')],
\]
where the kernel is Gaussian, 
\(
k(z,z') = \exp\!\Big(-\frac{\|z-z'\|^2}{2\sigma^2}\Big),
\)
and $\sigma$ is determined by the median heuristic on the pooled sample.
\end{itemize}

 \subsection{Additional results}\label{app:additional_results}

\subsubsection{Additional diagnostics for the main Scenarios (1-6)}
\begin{table}[H]
\centering
\caption{\textbf{Additional diagnostics for $Y$ and joint $Z=(X,Y)$.}
{\small \\ Smaller is better. Entries are mean (standard error) over $R=50$ replications.}}
\label{tab:appendix_tv_proj_mmd_all}
\renewcommand{\arraystretch}{1.2}
\resizebox{\textwidth}{!}{%
\begin{tabular}{@{}llccccc@{}}
\toprule
\textbf{DGP type} & \textbf{Model} & \textbf{TV $Y$ (↓)} & \textbf{Proj-TV $Z$ (↓)} & \textbf{Proj-Hellinger $Z$ (↓)} & \textbf{Proj-KL $Z$ (↓)} & \textbf{$\mathrm{MMD}^2$ $Z$} \\
\midrule\midrule
\multirow{7}{*}{1- linear}
& TWFE                & 0.49 (0.02) & 0.47 (0.01) & 0.46 (0.01) & 4.20 (0.33) & 0.28 (0.02) \\
& MatchSynth          & 0.45 (0.07) & 0.44 (0.05) & 0.43 (0.04) & 2.89 (1.02) & 0.24 (0.07) \\
& GenSynth            & 0.82 (0.03) & 0.75 (0.01) & 0.73 (0.01) & 13.13 (0.65) & 0.72 (0.04) \\
& GANSynth            & 0.74 (0.03) & 0.61 (0.02) & 0.59 (0.02) & 9.00 (0.63) & 0.56 (0.04) \\
\rowcolor[HTML]{E8F5E9}
& OTSynth (linear)    & \textbf{0.14 (0.04)} & \textbf{0.17 (0.03)} & \textbf{0.19 (0.02)} & \textbf{0.38 (0.09)} & \textbf{0.01 (0.01)} \\
\rowcolor[HTML]{E8F5E9}
& OTSynth (n.net)     & 0.22 (0.05) & 0.25 (0.04) & 0.26 (0.04) & 0.87 (0.38) & 0.05 (0.03) \\
\midrule\midrule
\multirow{7}{*}{2- smooth nonlinear}
& TWFE                & 0.53 (0.03) & 0.43 (0.02) & 0.42 (0.02) & 2.77 (0.34) & 0.32 (0.03) \\
& MatchSynth          & 0.67 (0.03) & 0.54 (0.02) & 0.52 (0.02) & 5.37 (0.58) & 0.51 (0.04) \\
& GenSynth            & 0.48 (0.06) & 0.60 (0.02) & 0.58 (0.02) & 8.18 (0.51) & 0.26 (0.04) \\
& GANSynth            & 0.29 (0.04) & 0.26 (0.02) & 0.27 (0.02) & 1.35 (0.30) & 0.08 (0.02) \\
\rowcolor[HTML]{E8F5E9}
& OTSynth (linear)    & \textbf{0.14 (0.03)} & \textbf{0.16 (0.01)} & \textbf{0.18 (0.01)} & \textbf{0.29 (0.05)} & \textbf{0.01 (0.01)} \\
\rowcolor[HTML]{E8F5E9}
& OTSynth (n.net)     & \textbf{0.14 (0.03)} & 0.18 (0.02) & 0.20 (0.01) & 0.38 (0.09) & \textbf{0.01 (0.01)} \\
\midrule\midrule
\multirow{7}{*}{3- strong nonlinear}
& TWFE                & 0.50 (0.02) & 0.40 (0.02) & 0.37 (0.02) & 1.59 (0.24) & 0.27 (0.03) \\
& MatchSynth          & 0.91 (0.01) & 0.75 (0.01) & 0.73 (0.01) & 11.56 (0.61) & 1.05 (0.05) \\
& GenSynth            & 0.70 (0.06) & 0.66 (0.02) & 0.64 (0.01) & 10.62 (0.46) & 0.44 (0.03) \\
& GANSynth            & 0.49 (0.03) & 0.33 (0.02) & 0.32 (0.02) & 1.38 (0.32) & 0.16 (0.02) \\
\rowcolor[HTML]{E8F5E9}
& OTSynth (linear)    & 0.75 (0.16) & 0.63 (0.17) & 0.61 (0.16) & 3.33 (2.83) & 0.59 (0.29) \\
\rowcolor[HTML]{E8F5E9}
& OTSynth (n.net)     & \textbf{0.30 (0.03)} & \textbf{0.23 (0.01)} & \textbf{0.23 (0.01)} & \textbf{0.45 (0.07)} & \textbf{0.02 (0.01)} \\
\midrule\midrule
\multirow{7}{*}{4- discontinuous}
& TWFE                & 0.53 (0.03) & 0.43 (0.02) & 0.42 (0.02) & 3.02 (0.37) & 0.31 (0.03) \\
& MatchSynth          & 0.73 (0.03) & 0.56 (0.02) & 0.54 (0.02) & 6.35 (0.60) & 0.59 (0.04) \\
& GenSynth            & 0.44 (0.06) & 0.61 (0.02) & 0.60 (0.02) & 9.17 (0.50) & 0.26 (0.03) \\
& GANSynth            & 0.47 (0.04) & 0.36 (0.02) & 0.36 (0.02) & 2.73 (0.44) & 0.21 (0.03) \\
\rowcolor[HTML]{E8F5E9}
& OTSynth (linear)    & \textbf{0.13 (0.03)} & \textbf{0.16 (0.01)} & \textbf{0.18 (0.01)} & \textbf{0.39 (0.08)} & \textbf{0.01 (0.01)} \\
\rowcolor[HTML]{E8F5E9}
& OTSynth (n.net)     & 0.18 (0.07) & 0.21 (0.04) & 0.22 (0.03) & 0.46 (0.11) & 0.03 (0.03) \\
\midrule\midrule
\multirow{7}{*}{5- linear, nonRCT}
& TWFE                & 0.24 (0.03) & 0.38 (0.01) & 0.37 (0.01) & 2.08 (0.20) & 0.20 (0.02) \\
& MatchSynth          & 0.30 (0.03) & 0.42 (0.01) & 0.42 (0.01) & 3.94 (0.29) & 0.25 (0.01) \\
& GenSynth            & \textbf{0.14 (0.02)} & 0.39 (0.01) & 0.40 (0.01) & 3.68 (0.18) & 0.19 (0.01) \\
& GANSynth            & 0.97 (0.01) & 0.84 (0.02) & 0.83 (0.02) & 17.79 (0.83) & 1.20 (0.04) \\
\rowcolor[HTML]{E8F5E9}
& OTSynth (linear)    & 0.23 (0.08) & \textbf{0.23 (0.05)} & \textbf{0.24 (0.04)} & \textbf{0.57 (0.22)} & \textbf{0.06 (0.04)} \\
\rowcolor[HTML]{E8F5E9}
& OTSynth (n.net)     & 0.30 (0.09) & 0.31 (0.05) & 0.31 (0.04) & 0.99 (0.31) & 0.12 (0.05) \\
\midrule\midrule
\multirow{7}{*}{6- linear, d=30}
& TWFE                & 0.70 (0.04) & 0.24 (0.01) & 0.24 (0.01) & 0.58 (0.07) & 0.11 (0.02) \\
& MatchSynth          & 0.69 (0.12) & 0.24 (0.04) & 0.25 (0.04) & 0.63 (0.25) & 0.12 (0.05) \\
& GenSynth            & 0.81 (0.06) & 0.63 (0.07) & 0.60 (0.06) & 8.15 (1.43) & 0.18 (0.04) \\
& GANSynth            & 0.53 (0.13) & 0.23 (0.04) & 0.24 (0.04) & 0.75 (0.39) & 0.08 (0.06) \\
\rowcolor[HTML]{E8F5E9}
& OTSynth (linear)    & 0.39 (0.04) & 0.19 (0.01) & 0.20 (0.01) & \textbf{0.43 (0.04)} & 0.03 (0.01) \\
\rowcolor[HTML]{E8F5E9}
& OTSynth (n.net)     & \textbf{0.17 (0.04)} & \textbf{0.16 (0.00)} & \textbf{0.18 (0.00)} & \textbf{0.39 (0.03)} & \textbf{0.01 (0.00)} \\
\bottomrule
\end{tabular}%
}
\end{table}

\subsubsection{Diagnostics for the additional robustness Scenarios (7-11)}
\begin{table}[H]
\centering
\caption[Marginal summaries of $Y$ for robustness scenarios]{\textbf{Marginal summaries of $Y$ across additional robustness scenarios.}
{\small \\ Closer to the Oracle is better. Entries are mean (standard error) over $R=50$ replications.}}
\label{tab:robust_y_summary}
\resizebox{\textwidth}{!}{%
\begin{tabular}{@{}llccccc@{}}
\toprule
\textbf{DGP type} & \textbf{Model} & \textbf{Mean} & \textbf{Std.\ dev} & \textbf{q1 (25\%)} & \textbf{q2 (median)} & \textbf{q3 (75\%)} \\
\midrule\midrule
\multirow{7}{*}{7- radial}
& TWFE                & 10.43 (0.29) & 3.18 (0.17) &  8.30 (0.31) & 10.41 (0.30) & 12.58 (0.33) \\
& MatchSynth          & 12.34 (1.35) & 2.05 (0.71) & 10.93 (1.46) & 12.32 (1.39) & 13.77 (1.49) \\
& {GenSynth}   & 10.46 (0.38) & \textbf{2.91 (0.51)} &  8.14 (1.10) & 10.29 (0.95) & 12.33 (0.77) \\
& GANSynth            & 17.41 (0.43) & 2.08 (0.17) & 16.04 (0.45) & 17.34 (0.47) & 18.72 (0.46) \\
\rowcolor[HTML]{E8F5E9}
& {OTSynth (linear)}    & \textbf{21.65 (0.69)} & 3.19 (0.23) & \textbf{19.52 (0.57)} & \textbf{21.66 (0.69)} & \textbf{23.79 (0.83)} \\
\rowcolor[HTML]{E8F5E9}
& OTSynth (n.net)     & 19.98 (0.68) & 2.45 (0.28) & 18.33 (0.64) & 19.97 (0.73) & 21.61 (0.81) \\
\rowcolor[HTML]{FFF3E0}
& \textbf{Oracle}     & 21.52 (0.13) & 2.84 (0.09) & 19.59 (0.15) & 21.50 (0.16) & 23.41 (0.16) \\
\midrule\midrule
\multirow{7}{*}{8- curvy}
& TWFE                &  1.90 (0.35) & 6.48 (0.21) & -2.22 (0.43) &  1.19 (0.34) &  5.51 (0.33) \\
& MatchSynth          & -1.72 (1.00) & 6.34 (0.72) & -5.56 (1.51) & -1.99 (1.42) &  1.91 (0.95) \\
& {GenSynth}   &  7.71 (0.35) & 3.59 (0.74) & \textbf{5.49 (1.01)} &  7.99 (0.93) & 10.67 (1.69) \\
& GANSynth            &  0.82 (0.51) & 4.34 (0.24) & -1.95 (0.60) &  0.80 (0.56) &  3.62 (0.53) \\
\rowcolor[HTML]{E8F5E9}
& {OTSynth (linear)}    & \textbf{8.95 (1.03)} & 6.80 (0.35) &  4.42 (0.97) & \textbf{8.96 (1.09)} & \textbf{13.54 (1.23)} \\
\rowcolor[HTML]{E8F5E9}
& {OTSynth (n.net)}     & 11.91 (1.57) & \textbf{7.55 (0.61)} &  6.82 (1.54) & 11.88 (1.73) & 17.01 (2.00) \\
\rowcolor[HTML]{FFF3E0}
& \textbf{Oracle}     & 10.15 (0.32) & 7.27 (0.26) &  5.23 (0.49) & 10.03 (0.43) & 14.97 (0.37) \\
\midrule\midrule
\multirow{7}{*}{9- smooth nonlinear, nonRCT}
& TWFE                & -7.69 (0.31) & 6.70 (0.20) & -12.21 (0.40) &  -7.78 (0.32) &  -3.25 (0.32) \\
& MatchSynth          & -11.20 (0.21)& 5.05 (0.22) & -14.59 (0.32) & -11.20 (0.29) &  -7.80 (0.33) \\
& GenSynth            & -10.32 (0.34)& 5.40 (0.18) & -14.02 (0.46) & -10.21 (0.41) &  -6.58 (0.47) \\
& GANSynth            & -15.83 (1.27)& 7.25 (0.67) & -20.89 (1.69) & -16.26 (1.46) & -11.03 (1.15) \\
\rowcolor[HTML]{E8F5E9}
& {OTSynth (linear)}    & -19.24 (0.60)& \textbf{8.49 (0.39)} & \textbf{-24.98 (0.70)} & -19.27 (0.65) & -13.50 (0.71) \\
\rowcolor[HTML]{E8F5E9}
& {OTSynth (n.net)}     & \textbf{-19.34 (0.97)}& 8.52 (0.66) & -24.93 (1.51) & \textbf{-19.53 (1.16)} & \textbf{-13.69 (0.94)} \\
\rowcolor[HTML]{FFF3E0}
& \textbf{Oracle}     & -20.27 (0.36)& 8.33 (0.27) & -25.88 (0.50) & -20.27 (0.42) & -14.62 (0.53) \\
\midrule\midrule
\multirow{7}{*}{10- smooth nonlinear, $d=30$}
& TWFE                & 19.23 (1.00) & 6.90 (0.24) & 14.59 (1.00) & 19.23 (0.98) & 23.91 (1.00) \\
& MatchSynth          & 18.95 (3.85) & 7.44 (0.50) & 13.96 (3.87) & 18.90 (3.85) & 23.97 (3.85) \\
& GenSynth            & 15.66 (1.81) & 4.33 (0.96) & 12.44 (2.68) & 15.69 (2.76) & 18.26 (2.70) \\
& GANSynth            & 16.57 (2.70) & 6.29 (0.54) & 12.36 (2.66) & 16.54 (2.71) & 20.83 (2.82) \\
\rowcolor[HTML]{E8F5E9}
& OTSynth (linear)    & 21.91 (0.90) & 8.39 (0.49) & 16.22 (0.90) & 21.92 (0.96) & 27.57 (1.10) \\
\rowcolor[HTML]{E8F5E9}
& {OTSynth (n.net)}     & \textbf{31.10 (1.03)} & \textbf{7.69 (0.44)} & \textbf{25.95 (0.98)} & \textbf{31.02 (1.09)} & \textbf{36.29 (1.21)} \\
\rowcolor[HTML]{FFF3E0}
& \textbf{Oracle}     & 31.80 (0.30) & 7.62 (0.23) & 26.66 (0.43) & 31.80 (0.44) & 36.98 (0.43) \\
\midrule\midrule
\multirow{7}{*}{11- linear, $d=30$, nonRCT}
& TWFE                &  5.11 (0.53) & 6.68 (0.29) &  0.59 (0.57) &  5.17 (0.52) &  9.63 (0.59) \\
& {MatchSynth} &  5.29 (0.21) & 6.84 (0.27) &  {0.71 (0.29)} &  {5.34 (0.25)} &  {9.89 (0.31)} \\
& {GenSynth}   &  4.83 (0.78) & 4.43 (0.72) &  \textbf{1.72 (1.49)} &  4.75 (1.25) &  7.58 (1.50) \\
& {GANSynth}   & \textbf{10.55 (3.42)} & 5.13 (0.50) &  7.07 (3.28) & \textbf{10.54 (3.47)} & \textbf{14.05 (3.56)} \\
\rowcolor[HTML]{E8F5E9}
& OTSynth (linear)    &  3.62 (1.38) & 7.99 (0.32) & -1.72 (1.45) &  3.67 (1.43) &  8.96 (1.42) \\
\rowcolor[HTML]{E8F5E9}
& {OTSynth (n.net)}     & 11.69 (1.05) & \textbf{7.19 (0.37)} &  6.89 (1.16) & 11.76 (1.11) & 16.56 (1.12) \\
\rowcolor[HTML]{FFF3E0}
& \textbf{Oracle}     &  8.01 (0.35) & 7.25 (0.23) &  3.09 (0.42) &  7.99 (0.38) & 12.92 (0.51) \\
\bottomrule
\end{tabular}%
}
\end{table}

% ===================== TABLE B: Distances (Y and joint Z) =====================
\begin{table}[H]
\centering
\caption[Distributional distances for $Y$ and joint $Z=(X,Y)$ (robustness scenarios)]{\textbf{Distributional distances for $Y$ and joint $(X,Y)$ (robustness scenarios).}
{\small \\ Smaller is better. Entries are mean (standard error) over $R=50$ replications.}}
\label{tab:robust_distances}
\resizebox{\textwidth}{!}{%
\begin{tabular}{@{}llccccc@{}}
\toprule
\textbf{DGP type} & \textbf{Model} & \textbf{W1 $Y$(↓)} & \textbf{Hellinger $Y$(↓)} & \textbf{KL Div.\ $Y$(↓)} & \textbf{Energy $Z$(↓)} & \textbf{Sliced W1 $Z$(↓)} \\
\midrule\midrule
\multirow{7}{*}{7- radial}
& TWFE                & 11.09 (0.33) & 0.92 (0.01) & 15.73 (2.65) & 12.51 (0.58) & 5.34 (0.15) \\
& MatchSynth          &  9.18 (1.36) & 0.92 (0.07) & 20.10 (5.01) &  9.71 (2.29) & 4.59 (0.58) \\
& GenSynth            & 11.06 (0.42) & 0.93 (0.02) & 17.70 (2.31) & 15.54 (0.67) & 5.52 (0.19) \\
& GANSynth            &  4.10 (0.46) & 0.57 (0.05) &  5.08 (2.09) &  2.57 (0.49) & 1.92 (0.20) \\
\rowcolor[HTML]{E8F5E9}
& OTSynth (linear)    & \textbf{0.66 (0.40)} & \textbf{0.16 (0.04)} & \textbf{0.17 (0.11)} & \textbf{0.11 (0.10)} & \textbf{0.45 (0.16)} \\
\rowcolor[HTML]{E8F5E9}
& OTSynth (n.net)     &  1.59 (0.60) & 0.27 (0.07) &  1.10 (0.85) &  0.54 (0.28) & 0.89 (0.23) \\
\midrule\midrule
\multirow{7}{*}{8- curvy}
& TWFE                &  8.26 (0.55) & 0.43 (0.03) &  1.12 (0.26) &  5.63 (0.65) & 4.20 (0.21) \\
& MatchSynth          & 11.87 (1.00) & 0.58 (0.03) &  2.97 (0.81) & 10.58 (1.32) & 5.61 (0.40) \\
& GenSynth            &  3.57 (0.64) & 0.52 (0.05) &  8.46 (1.54) &  4.18 (0.43) & 2.90 (0.17) \\
& GANSynth            &  9.33 (0.62) & 0.57 (0.03) &  7.18 (1.50) &  7.49 (0.89) & 4.45 (0.29) \\
\rowcolor[HTML]{E8F5E9}
& OTSynth (linear)    & \textbf{1.47 (0.79)} & \textbf{0.16 (0.03)} & {0.36 (0.20)} & \textbf{0.24 (0.23)} & \textbf{0.75 (0.34)} \\
\rowcolor[HTML]{E8F5E9}
& OTSynth (n.net)     &  1.99 (1.41) & 0.18 (0.04) &  \textbf{0.27 (0.12)} &  0.60 (0.59) & 1.09 (0.58) \\
\midrule\midrule
\multirow{7}{*}{9- smooth nonlinear, nonRCT}
& TWFE                & 12.57 (0.53) & 0.57 (0.02) &  4.47 (1.17) & 11.12 (0.81) & 6.72 (0.23) \\
& MatchSynth          &  9.07 (0.44) & 0.51 (0.02) &  4.95 (1.32) &  7.69 (0.61) & 5.38 (0.18) \\
& GenSynth            &  9.96 (0.48) & 0.53 (0.02) &  6.43 (1.18) &  8.91 (0.66) & 5.41 (0.21) \\
& GANSynth            &  4.45 (1.29) & 0.26 (0.06) &  1.24 (0.84) &  1.65 (0.92) & 2.16 (0.56) \\
\rowcolor[HTML]{E8F5E9}
& OTSynth (linear)    & \textbf{1.21 (0.55)} & \textbf{0.14 (0.02)} & \textbf{0.18 (0.12)} & \textbf{0.24 (0.11)} & \textbf{0.76 (0.18)} \\
\rowcolor[HTML]{E8F5E9}
& OTSynth (n.net)     &  1.44 (0.61) & 0.16 (0.02) &  0.21 (0.12) &  0.58 (0.17) & 1.19 (0.16) \\
\midrule\midrule
\multirow{7}{*}{10- smooth nonlinear, $d=30$}
& TWFE                & 12.58 (1.04) & 0.61 (0.04) &  3.80 (1.18) &  2.95 (0.06) & 2.95 (0.06) \\
& MatchSynth          & 12.86 (3.85) & 0.59 (0.13) &  3.61 (2.69) &  5.70 (3.10) & 3.02 (0.24) \\
& GenSynth            & 16.15 (1.88) & 0.86 (0.04) & 18.23 (1.74) & 13.19 (3.18) & 2.80 (0.31) \\
& GANSynth            & 15.23 (2.70) & 0.69 (0.07) &  8.84 (3.72) &  8.59 (3.43) & 2.31 (0.40) \\
\rowcolor[HTML]{E8F5E9}
& OTSynth (linear)    &  9.90 (0.94) & 0.47 (0.04) &  1.58 (0.73) &  3.25 (0.58) & 1.45 (0.13) \\
\rowcolor[HTML]{E8F5E9}
& OTSynth (n.net)     & \textbf{1.21 (0.64)} & \textbf{0.13 (0.02)} & \textbf{0.19 (0.17)} & \textbf{0.29 (0.07)} & \textbf{0.43 (0.05)} \\
\midrule\midrule
\multirow{7}{*}{11- linear, $d=30$, nonRCT}
& TWFE                &  2.90 (0.56) & 0.19 (0.02) & 0.33 (0.16) &  9.47 (0.14) & 3.51 (0.02) \\
& MatchSynth          &  \textbf{2.72 (0.35)} & \textbf{0.18 (0.01)} & \textbf{0.28 (0.13)} &  9.42 (0.10) & 3.51 (0.02) \\
& GenSynth            &  3.81 (0.78) & 0.44 (0.05) & 4.12 (0.97) & 12.70 (1.16) & 2.85 (0.12) \\
& GANSynth            &  3.97 (1.82) & 0.31 (0.08) & 1.96 (1.20) & 15.06 (2.49) & 3.16 (0.33) \\
\rowcolor[HTML]{E8F5E9}
& OTSynth (linear)    &  4.40 (1.44) & 0.25 (0.06) & 0.43 (0.32) &  \textbf{2.01 (0.53)} & \textbf{1.13 (0.15)} \\
\rowcolor[HTML]{E8F5E9}
& OTSynth (n.net)     &  3.70 (1.17) & 0.23 (0.05) & 0.47 (0.28) & 12.21 (0.70) & 3.00 (0.11) \\
\bottomrule
\end{tabular}%
}
\end{table}

% ===================== TABLE C: TV(Y) + Projection diagnostics (Z) =====================
\begin{table}[H]
\centering
\caption{\textbf{Additional diagnostics for $Y$ and joint $Z=(X,Y)$.}
{\small \\ Smaller is better. Entries are mean (standard error) over $R=50$ replications.}}
\label{tab:robust_tv_proj}
\resizebox{\textwidth}{!}{%
\begin{tabular}{@{}llccccc@{}}
\toprule
\textbf{DGP type} & \textbf{Model} & \textbf{TV $Y$ (↓)} & \textbf{Proj-TV $Z$ (↓)} & \textbf{Proj-Hellinger $Z$ (↓)} & \textbf{Proj-KL $Z$ (↓)} & \textbf{$\mathrm{MMD}^2$ $Z$} \\
\midrule\midrule
\multirow{7}{*}{7- radial}
& TWFE                & 0.94 (0.01) & 0.57 (0.01) & 0.56 (0.01) &  6.10 (0.45) & 0.72 (0.03) \\
& MatchSynth          & 0.93 (0.06) & 0.53 (0.05) & 0.52 (0.04) &  6.17 (1.37) & 0.62 (0.12) \\
& GenSynth            & 0.94 (0.02) & 0.77 (0.01) & 0.75 (0.01) & 13.16 (0.68) & 0.88 (0.04) \\
& GANSynth            & 0.61 (0.05) & 0.33 (0.03) & 0.33 (0.02) &  1.97 (0.40) & 0.21 (0.04) \\
\rowcolor[HTML]{E8F5E9}
& OTSynth (linear)    & \textbf{0.15 (0.04)} & \textbf{0.16 (0.01)} & \textbf{0.18 (0.01)} & \textbf{0.29 (0.05)} & \textbf{0.01 (0.01)} \\
\rowcolor[HTML]{E8F5E9}
& OTSynth (n.net)     & 0.27 (0.08) & 0.22 (0.03) & 0.23 (0.02) &  0.68 (0.22) & 0.04 (0.02) \\
\midrule\midrule
\multirow{7}{*}{8- curvy}
& TWFE                & 0.49 (0.03) & 0.41 (0.02) & 0.38 (0.02) &  1.53 (0.18) & 0.27 (0.03) \\
& MatchSynth          & 0.65 (0.03) & 0.54 (0.02) & 0.50 (0.02) &  3.64 (0.41) & 0.46 (0.05) \\
& GenSynth            & 0.50 (0.07) & 0.64 (0.02) & 0.62 (0.02) &  9.55 (0.60) & 0.30 (0.05) \\
& GANSynth            & 0.61 (0.04) & 0.48 (0.02) & 0.47 (0.02) &  4.83 (0.65) & 0.38 (0.04) \\
\rowcolor[HTML]{E8F5E9}
& OTSynth (linear)    & \textbf{0.14 (0.03)} & \textbf{0.17 (0.02)} & \textbf{0.19 (0.02)} & \textbf{0.51 (0.14)} & \textbf{0.01 (0.01)} \\
\rowcolor[HTML]{E8F5E9}
& OTSynth (n.net)     & 0.17 (0.05) & 0.21 (0.03) & 0.22 (0.03) &  0.53 (0.11) & 0.03 (0.03) \\
\midrule\midrule
\multirow{7}{*}{9- smooth nonlinear, nonRCT}
& TWFE                & 0.60 (0.02) & 0.53 (0.02) & 0.51 (0.02) &  4.16 (0.52) & 0.43 (0.03) \\
& MatchSynth          & 0.53 (0.03) & 0.49 (0.02) & 0.47 (0.02) &  4.33 (0.59) & 0.36 (0.03) \\
& GenSynth            & 0.55 (0.03) & 0.54 (0.02) & 0.54 (0.01) &  7.14 (0.55) & 0.39 (0.03) \\
& GANSynth            & 0.24 (0.07) & 0.25 (0.04) & 0.27 (0.04) &  1.34 (0.58) & 0.07 (0.04) \\
\rowcolor[HTML]{E8F5E9}
& OTSynth (linear)    & \textbf{0.12 (0.02)} & \textbf{0.17 (0.01)} & \textbf{0.19 (0.01)} & \textbf{0.38 (0.10)} & \textbf{0.01 (0.00)} \\
\rowcolor[HTML]{E8F5E9}
& OTSynth (n.net)     & 0.15 (0.03) & 0.21 (0.02) & 0.23 (0.01) &  0.63 (0.15) & 0.03 (0.01) \\
\midrule\midrule
\multirow{7}{*}{10- smooth nonlinear, $d=30$}
& TWFE                & 0.61 (0.04) & 0.24 (0.01) & 0.24 (0.01) & 0.59 (0.07) & 0.10 (0.02) \\
& MatchSynth          & 0.59 (0.13) & 0.24 (0.04) & 0.24 (0.04) & 0.61 (0.28) & 0.11 (0.06) \\
& GenSynth            & 0.86 (0.04) & 0.66 (0.07) & 0.63 (0.06) & 9.21 (1.53) & 0.26 (0.05) \\
& GANSynth            & 0.72 (0.07) & 0.29 (0.03) & 0.30 (0.03) & 1.25 (0.49) & 0.17 (0.06) \\
\rowcolor[HTML]{E8F5E9}
& OTSynth (linear)    & 0.47 (0.04) & 0.22 (0.01) & 0.23 (0.01) & 0.55 (0.07) & 0.06 (0.01) \\
\rowcolor[HTML]{E8F5E9}
& OTSynth (n.net)     & \textbf{0.13 (0.02)} & \textbf{0.16 (0.00)} & \textbf{0.17 (0.00)} & \textbf{0.37 (0.03)} & \textbf{0.00 (0.00)} \\
\midrule\midrule
\multirow{7}{*}{11- linear, $d=30$, nonRCT}
& TWFE                & 0.19 (0.03) & 0.31 (0.00) & 0.31 (0.00) & 1.19 (0.05) & 0.19 (0.00) \\
& MatchSynth          & \textbf{0.17 (0.02)} & 0.31 (0.00) & 0.31 (0.00) & 1.18 (0.04) & 0.19 (0.00) \\
& GenSynth            & 0.45 (0.07) & 0.57 (0.04) & 0.55 (0.04) & 7.10 (0.68) & 0.26 (0.02) \\
& GANSynth            & 0.30 (0.09) & 0.39 (0.03) & 0.40 (0.02) & 3.46 (0.56) & 0.30 (0.04) \\
\rowcolor[HTML]{E8F5E9}
& OTSynth (linear)    & 0.25 (0.06) & \textbf{0.19 (0.01)} & \textbf{0.21 (0.01)} & \textbf{0.47 (0.06)} & \textbf{0.04 (0.01)} \\
\rowcolor[HTML]{E8F5E9}
& OTSynth (n.net)     & 0.22 (0.06) & 0.35 (0.01) & 0.35 (0.01) & 1.96 (0.18) & 0.23 (0.01) \\
\bottomrule
\end{tabular}%
}
\end{table}

\begin{figure}[H]
\centering
\setlength{\tabcolsep}{1pt}
\renewcommand{\arraystretch}{0.9}

\begin{tabular}{@{}m{0.12\textwidth}*{6}{>{\centering\arraybackslash}m{0.145\textwidth}}@{}}
 & {7- radial} & {8- curvy} & {9- smooth, nonRCT} & {10- smooth, d=30} & {11- linear, nonRCT, d=30} \\

{TWFE}
  & \simcell{scenario3_radial}{output_twfe}
  & \simcell{scenario4_curvy}{output_twfe}
  & \simcell{scenario7_smooth_nonRCT}{output_twfe}
  & \simcell{scenario9_smooth_highdim}{output_twfe}
  & \simcell{scenariot_linear_nonRCT_highdim}{output_twfe} \\

{Match Synth}
  & \simcell{scenario3_radial}{output_match}
  & \simcell{scenario4_curvy}{output_match}
  & \simcell{scenario7_smooth_nonRCT}{output_match}
  & \simcell{scenario9_smooth_highdim}{output_match}
  & \simcell{scenariot_linear_nonRCT_highdim}{output_match} \\

{Gen$\;$ Synth}
  & \simcell{scenario3_radial}{output_gen}
  & \simcell{scenario4_curvy}{output_gen}
  & \simcell{scenario7_smooth_nonRCT}{output_gen}
  & \simcell{scenario9_smooth_highdim}{output_gen}
  & \simcell{scenariot_linear_nonRCT_highdim}{output_gen} \\

{Gan$\;$ Synth}
  & \simcell{scenario3_radial}{output_gan}
  & \simcell{scenario4_curvy}{output_gan}
  & \simcell{scenario7_smooth_nonRCT}{output_gan}
  & \simcell{scenario9_smooth_highdim}{output_gan}
  & \simcell{scenariot_linear_nonRCT_highdim}{output_gan} \\

{OTSynth (linear)}
  & \simcell{scenario3_radial}{output_ot_lin}
  & \simcell{scenario4_curvy}{output_ot_lin}
  & \simcell{scenario7_smooth_nonRCT}{output_ot_lin}
  & \simcell{scenario9_smooth_highdim}{output_ot_lin}
  & \simcell{scenariot_linear_nonRCT_highdim}{output_ot_lin} \\

{OTSynth (n.net)}
  & \simcell{scenario3_radial}{output_ot_nnet}
  & \simcell{scenario4_curvy}{output_ot_nnet}
  & \simcell{scenario7_smooth_nonRCT}{output_ot_nnet}
  & \simcell{scenario9_smooth_highdim}{output_ot_nnet}
  & \simcell{scenariot_linear_nonRCT_highdim}{output_ot_nnet} \\

{oracle$\;$ map}
  & \simcellt{scenario3_radial}{output_T}
  & \simcellt{scenario4_curvy}{output_T}
  & \simcellt{scenario7_smooth_nonRCT}{output_T}
  & \simcellt{scenario2_smooth}{output_T}
  & \simcellt{scenario5_linear_nonRCT}{output_T} \\
\end{tabular}

\caption{Comparison of synthesized target–site treatments across robustness scenarios (columns) and methods (rows). Orange points show the synthesized $Z_1^{\prime\,(\mathrm{synth.})}$; blue points show the oracle $Z_1'$.For the higher-dimensional ($d=30$) settings, the first two principal components of features $X$ are shown along with response $Y$, to enable 3D visualization.}
\label{fig: additional_scenarios}
\end{figure}
 
\bibliographystyle{chicago} 
\bibliography{refs} 

\end{document}
